# Supplementary material for: Controller Design and Implementation of a New Quadrotor Manipulation System
Source: arXiv:1904.08498 source file (2025-09-04)
Supplement: Supplementary file 1 [file Appendix_invkin.tex]

\chapter{Inverse Kinematics} \label{app:inversekinematics}

% change according to folder and file names
\ifpdf
    \graphicspath{{10_Appendices/figures/PNG/}{10_Appendices/figures/PDF/}{10_Appendices/figures/}}
\else
    \graphicspath{{10_Appendices/figures/EPS/}{10_Appendices/figures/}}
\fi
% ----------------------- contents from here ------------------------
\lstset {language=Matlab} 
\begin{lstlisting}
function zt_des = Inverse_Kin(Xe_des,sb)
L0 = 30e-03;
L1 = 70e-03;
L2 = 85e-03; 

xe=Xe_des(1);
ye=Xe_des(2);
ze=Xe_des(3);
epe=Xe_des(4);
the=Xe_des(5);
phe=Xe_des(6);
ph = sb(2);
th = sb(1);

T_end = [ cos(epe)*cos(the), cos(epe)*sin(phe)*sin(the) - cos(phe)*sin(epe),
 sin(epe)*sin(phe) + cos(epe)*cos(phe)*sin(the);
cos(the)*sin(epe), cos(epe)*cos(phe) + sin(epe)*sin(phe)*sin(the),
 cos(phe)*sin(epe)*sin(the) - cos(epe)*sin(phe);
-sin(the),     cos(the)*sin(phe),cos(phe)*cos(the)];                                                  										

r11 = T_end(1,1);
r12 = T_end(1,2);
r13 = T_end(1,3);
r23 = T_end(2,3);
r31 = T_end(3,1);
r32 = T_end(3,2);
r33 = T_end(3,3);


a1=cos(ph)*cos(th);
b1=cos(th)*sin(ph);
if(((-2*b1)^2 - 4*(-a1-r33)*(a1-r33))<0)
t2=0;   
else
% t1=(-(-2*b1) + sqrt((-2*b1)^2 - 4*(-a1-r33)*(a1-r33)))/(2*(-a1-r33));
t2=(-(-2*b1) -sqrt((-2*b1)^2 - 4*(-a1-r33)*(a1-r33)))/(2*(-a1-r33));
% th1=2*atan(t1)
% OR
end
th1=2*atan(t2);
%% Case#2 ====>> Sin(th1) = 0
if(th1<=0.0001&&th1>=-0.0001)
th1=0;
ep=0;
a6=cos(th)*cos(ep);
b6=cos(ph)*sin(ep)-sin(ph)*sin(th)*cos(ep);
a7=sin(ph)*sin(th)*cos(ep)-cos(ph)*sin(ep);
b7=cos(th)*cos(ep);
sth2=(b7*r11+b6*r12)/(a6*b7+a7*b6);
cth2=(a7*r11+a6*r12)/(a6*b7+a7*b6);
th2=atan2(sth2,cth2);
%% Case#3 ====>> Sin(th1) = pi
elseif (th1==pi)
th1=pi;
ep=0;
a6=cos(th)*cos(ep);
b6=-cos(ph)*sin(ep)+sin(ph)*sin(th)*cos(ep);
a7=-sin(ph)*sin(th)*cos(ep)+cos(ph)*sin(ep);
b7=cos(th)*cos(ep);
sth2=(b7*r11+b6*r12)/(a6*b7+a7*b6);
cth2=(a7*r11+a6*r12)/(a6*b7+a7*b6);
th2=atan2(sth2,cth2);
%% Case#1 ====>> Sin(th1) != 0 ======>> r13~=0 && r23 ~=0    
else
a2=cos(ph)*sin(th1)+sin(ph)*cos(th1);
b2=cos(ph)*sin(th)*cos(th1)-sin(ph)*sin(th)*sin(th1);

a3=cos(ph)*sin(th)*cos(th1)-sin(ph)*sin(th)*sin(th1);
b3=-sin(ph)*cos(th1)-cos(ph)*sin(th1);

a4=cos(ph)*cos(th)*sin(th1)+cos(th)*sin(ph)*cos(th1);
b4=-sin(th);

a5=-sin(th);
b5=-cos(ph)*cos(th)*sin(th1)-cos(th)*sin(ph)*cos(th1);

sep=(b3*r13+b2*r23)/(a2*b3+a3*b2);
cep=(a3*r13+a2*r23)/(a2*b3+a3*b2);
ep=atan2(sep,cep);
sth2=(b5*r32+b4*r31)/(a4*b5+a5*b4);
cth2=(a5*r32+a4*r31)/(a4*b5+a5*b4);
th2=atan2(sth2,cth2);
end
%% Translational Part
X=xe- (- L0*(sin(ph)*sin(ep) + cos(ph)*sin(th)*cos(ep)) +
 L2*cos(th2)*(cos(th1)*(cos(ph)*sin(ep) - sin(ph)*sin(th)*cos(ep)) -
  sin(th1)*(sin(ph)*sin(ep) + cos(ph)*sin(th)*cos(ep))) +
   L1*cos(th1)*(cos(ph)*sin(ep) - sin(ph)*sin(th)*cos(ep)) -
    L1*sin(th1)*(sin(ph)*sin(ep) + cos(ph)*sin(th)*cos(ep)) +
     L2*cos(th)*cos(ep)*sin(th2));
Y=ye- (+ L0*(sin(ph)*cos(ep) - cos(ph)*sin(th)*sin(ep)) -
 L2*cos(th2)*(cos(th1)*(cos(ph)*cos(ep) + sin(ph)*sin(th)*sin(ep)) -
  sin(th1)*(sin(ph)*cos(ep) - cos(ph)*sin(th)*sin(ep))) -
   L1*cos(th1)*(cos(ph)*cos(ep) + sin(ph)*sin(th)*sin(ep)) +
    L1*sin(th1)*(sin(ph)*cos(ep) - cos(ph)*sin(th)*sin(ep)) +
     L2*cos(th)*sin(ep)*sin(th2));
Z=ze- (- L2*sin(th)*sin(th2) - L0*cos(ph)*cos(th) -
 L2*cos(th2)*(cos(ph)*cos(th)*sin(th1) + cos(th)*sin(ph)*cos(th1)) -
  L1*cos(ph)*cos(th)*sin(th1) - L1*cos(th)*sin(ph)*cos(th1));
%% ==========
zt_des=[X;Y;Z;ep;th1;th2];
end

\end{lstlisting}
