# Supplementary material for: Controller Design and Implementation of a New Quadrotor Manipulation System
Source: arXiv:1904.08498 source file (2025-09-04)
Supplement: Supplementary file 2 [file Appendix_jacob.tex]

\chapter{System Jacobian and Parametrization} \label{app:system_Jacobian} 

% change according to folder and file names
\ifpdf
    \graphicspath{{10_Appendices/figures/PNG/}{10_Appendices/figures/PDF/}{10_Appendices/figures/}}
\else
    \graphicspath{{10_Appendices/figures/EPS/}{10_Appendices/figures/}}
\fi

% ----------------------- contents from here ------------------------
The coding of the system Jacobian is given as following.
\lstset {language=Matlab, breaklines=true} 
\begin{lstlisting}
function [Jz,Js,TAe] = jacob(Xdde_ref,zt,ztd,sb,sbd,Xe,sbdd,Jzd,Jsd,TAed,Xde)
L0 = 30e-03 ;
L1 = 70e-03;
L2 = 85e-03;

X=zt(1);
Y=zt(2);
Z=zt(3);
ep=zt(4);
th1=zt(5);
th2=zt(6);

ph=sb(2);
th=sb(1);

phd=sbd(2);
thd=sbd(1);

xe=Xe(1);
ye=Xe(2);
ze=Xe(3);
epe=Xe(4);
the=Xe(5);
phe=Xe(6);
%% ===================
I3=eye(3); O3=zeros(3);
A0_B = [0 0 1 0; -1 0 0 0; 0 -1 0 -L0; 0 0 0 1]; 
A1_0 = [cos(th1) 0 sin(th1) L1*cos(th1); sin(th1) 0 -cos(th1) L1*sin(th1); 
0 1 0 0; 0 0 0 1]; 
A2_1 = [cos(th2) -sin(th2) 0 L2*cos(th2); sin(th2) cos(th2) 0 L2*sin(th2); 
0 0 1 0; 0 0 0 1];

Rb_I = [cos(ep)*cos(th), cos(ep)*sin(ph)*sin(th)-cos(ph)*sin(ep),
 sin(ep)*sin(ph)+cos(ep)*cos(ph)*sin(th);
cos(th)*sin(ep), cos(ep)*cos(ph)+sin(ep)*sin(ph)*sin(th),
 cos(ph)*sin(ep)*sin(th)-cos(ep)*sin(ph);
-sin(th), cos(th)*sin(ph), cos(ph)*cos(th)];

R0_B=A0_B(1:3,1:3);
R1_0=A1_0(1:3,1:3);
RB_I=Rb_I;
%
a1=L1; d1=0; 
a2=L2; d2=0; 
z0=eye(3)*[0;0;1];z1=R1_0*[0;0;1];
r1_0=[a1*cos(th1);a1*sin(th1);d1];
r2_1=[a2*cos(th2);a2*sin(th2);d2];
p2_2=[0;0;0];
p2_1=R1_0*r2_1+p2_2;
p2_0=eye(3)*r1_0+p2_1;
alpha1=cross(z0,p2_0);
beta1=z0;
alpha2=cross(z1,p2_1);
beta2=z1;
A2_B=A0_B*A1_0*A2_1;
peb_b=A2_B(1:3,4);
Jt=[R0_B*alpha1,R0_B*alpha2];
Jr=[R0_B*beta1,R0_B*beta2];
Jeb_b=[Jt;Jr];
Rb=RB_I;
Tb=[0,-sin(ep),cos(ep)*cos(th);
0,cos(ep),sin(ep)*cos(th);
1,0,-sin(th)];
TAb=[I3,O3;O3,Tb];
Jb=[I3,-skew(Rb*peb_b);O3,I3];
Jeb=[Rb,O3;O3,Rb]*Jeb_b;
JbA=Jb*TAb;
Jet=JbA(:,1:4);
Jz=[Jet,Jeb];
Js=JbA(:,5:6);
Te=[0,-sin(epe),cos(epe)*cos(the);
0,cos(epe),sin(epe)*cos(the);
1,0,-sin(the)];
TAe=[I3,O3;O3,Te];
end
\end{lstlisting}

The details and coding of the regressor matrices, $Y_w$, $Y_e$, $Y_l$, $Y_i$, and $Y_s$, are given as following.
\lstset {language=Matlab, breaklines=true} 
\begin{lstlisting}
syms ph th ep th1 th2 xd yd zd phd thd epd thd1 thd2 xdd ydd zdd phdd thdd epdd thdd1 thdd2
syms mb m1 m2 Ix Iy Iz I1 I2 L0 L1 L2 g f1 f2 f3 f4 Tm1 Tm2 d c
syms L0m1 L0m2 L1m1 L1m2 L2m1 L2m2 L02m1 L02m2 L12m1 L12m2 L22m1 L22m2
syms L0L1m1  L0L1m2  L1L2m1  L1L2m2  L0L2m1  L0L2m2 zzz
% x=sym('x','real'); y=sym('y','real'); z=sym('z','real');
ph=sym('ph','real'); th=sym('th','real'); ep=sym('ep','real');
th1=sym('th1','real'); th2=sym('th2','real'); 
L0=sym('L0','real');L1=sym('L1','real'); L2=sym('L2','real'); 
mb=sym('mb','real');m1=sym('m1','real'); m2=sym('m2','real');
I1=sym('I1','real'); I2=sym('I2','real'); Ix=sym('Ix','real');
g=sym('g','real'); 

xd=sym('xd','real'); yd=sym('yd','real'); zd=sym('zd','real');
phd=sym('phd','real'); thd=sym('thd','real'); epd=sym('epd','real');
thd1=sym('thd1','real'); thd2=sym('thd2','real');

xdd=sym('xdd','real'); ydd=sym('ydd','real'); zdd=sym('zdd','real');
phdd=sym('phdd','real'); thdd=sym('thdd','real'); epdd=sym('epdd','real');
thdd1=sym('thdd1','real'); thdd2=sym('thdd2','real');
%% ====================================================
load('Mqdd_Cqd_G.mat');

TH = [m1;m2;mb;I1;I2;Ix;L0*m1;L0*m2;L1*m1;L1*m2;L2*m1;L2*m2;L0^2*m1;L0^2*m2;L1^2*m1;L1^2*m2;L2^2*m1;L2^2*m2;L0*L1*m1;L0*L1*m2;L1*L2*m1;L1*L2*m2;L0*L2*m1;L0*L2*m2];

Y1_TH = zzz*ones(size(TH'))*TH + Mqdd_Cqd_G(1);
Y2_TH = zzz*ones(size(TH'))*TH + Mqdd_Cqd_G(2);
Y3_TH = zzz*ones(size(TH'))*TH + Mqdd_Cqd_G(3);
Y4_TH = zzz*ones(size(TH'))*TH + Mqdd_Cqd_G(4);
Y5_TH = zzz*ones(size(TH'))*TH + Mqdd_Cqd_G(5);
Y6_TH = zzz*ones(size(TH'))*TH + Mqdd_Cqd_G(6);
Y7_TH = zzz*ones(size(TH'))*TH + Mqdd_Cqd_G(7);
Y8_TH = zzz*ones(size(TH'))*TH + Mqdd_Cqd_G(8);

Y1_TH=subs(Y1_TH,[L0*L1*m1,L0*L1*m2,L1*L2*m1,L1*L2*m2,L0*L2*m1,L0*L2*m2,L0^2*m1,L0^2*m2,L1^2*m1,L1^2*m2,L2^2*m1,L2^2*m2,L0*m1,L0*m2,L1*m1,L1*m2,L2*m1,L2*m2] ...
,[L0L1m1  ,L0L1m2  ,L1L2m1  ,L1L2m2  ,L0L2m1  ,L0L2m2  ,L02m1  ,L02m2  ,L12m1  ,L12m2  ,L22m1  ,L22m2  ,L0m1 ,L0m2 ,L1m1 ,L1m2 ,L2m1 ,L2m2]);
[cy1,ty1] = coeffs(Y1_TH, [m1,m2,mb,I1,I2,Ix,L0m1,L0m2,L1m1,L1m2,L2m1,L2m2,L02m1,L02m2,L12m1,L12m2,L22m1,L22m2,L0L1m1,L0L1m2,L1L2m1,L1L2m2,L0L2m1,L0L2m2]);
%===================================
Y2_TH=subs(Y2_TH,[L0*L1*m1,L0*L1*m2,L1*L2*m1,L1*L2*m2,L0*L2*m1,L0*L2*m2,L0^2*m1,L0^2*m2,L1^2*m1,L1^2*m2,L2^2*m1,L2^2*m2,L0*m1,L0*m2,L1*m1,L1*m2,L2*m1,L2*m2] ...
,[L0L1m1  ,L0L1m2  ,L1L2m1  ,L1L2m2  ,L0L2m1  ,L0L2m2  ,L02m1  ,L02m2  ,L12m1  ,L12m2  ,L22m1  ,L22m2  ,L0m1 ,L0m2 ,L1m1 ,L1m2 ,L2m1 ,L2m2]);
[cy2,ty2] = coeffs(Y2_TH, [m1,m2,mb,I1,I2,Ix,L0m1,L0m2,L1m1,L1m2,L2m1,L2m2,L02m1,L02m2,L12m1,L12m2,L22m1,L22m2,L0L1m1,L0L1m2,L1L2m1,L1L2m2,L0L2m1,L0L2m2]);
%===================================
Y3_TH=subs(Y3_TH,[L0*L1*m1,L0*L1*m2,L1*L2*m1,L1*L2*m2,L0*L2*m1,L0*L2*m2,L0^2*m1,L0^2*m2,L1^2*m1,L1^2*m2,L2^2*m1,L2^2*m2,L0*m1,L0*m2,L1*m1,L1*m2,L2*m1,L2*m2] ...
,[L0L1m1  ,L0L1m2  ,L1L2m1  ,L1L2m2  ,L0L2m1  ,L0L2m2  ,L02m1  ,L02m2  ,L12m1  ,L12m2  ,L22m1  ,L22m2  ,L0m1 ,L0m2 ,L1m1 ,L1m2 ,L2m1 ,L2m2]);
[cy3,ty3] = coeffs(Y3_TH, [m1,m2,mb,I1,I2,Ix,L0m1,L0m2,L1m1,L1m2,L2m1,L2m2,L02m1,L02m2,L12m1,L12m2,L22m1,L22m2,L0L1m1,L0L1m2,L1L2m1,L1L2m2,L0L2m1,L0L2m2]);
%===================================
Y4_TH=subs(Y4_TH,[L0*L1*m1,L0*L1*m2,L1*L2*m1,L1*L2*m2,L0*L2*m1,L0*L2*m2,L0^2*m1,L0^2*m2,L1^2*m1,L1^2*m2,L2^2*m1,L2^2*m2,L0*m1,L0*m2,L1*m1,L1*m2,L2*m1,L2*m2] ...
,[L0L1m1  ,L0L1m2  ,L1L2m1  ,L1L2m2  ,L0L2m1  ,L0L2m2  ,L02m1  ,L02m2  ,L12m1  ,L12m2  ,L22m1  ,L22m2  ,L0m1 ,L0m2 ,L1m1 ,L1m2 ,L2m1 ,L2m2]);
[cy4,ty4] = coeffs(Y4_TH, [m1,m2,mb,I1,I2,Ix,L0m1,L0m2,L1m1,L1m2,L2m1,L2m2,L02m1,L02m2,L12m1,L12m2,L22m1,L22m2,L0L1m1,L0L1m2,L1L2m1,L1L2m2,L0L2m1,L0L2m2]);
%===================================
Y5_TH=subs(Y5_TH,[L0*L1*m1,L0*L1*m2,L1*L2*m1,L1*L2*m2,L0*L2*m1,L0*L2*m2,L0^2*m1,L0^2*m2,L1^2*m1,L1^2*m2,L2^2*m1,L2^2*m2,L0*m1,L0*m2,L1*m1,L1*m2,L2*m1,L2*m2] ...
,[L0L1m1  ,L0L1m2  ,L1L2m1  ,L1L2m2  ,L0L2m1  ,L0L2m2  ,L02m1  ,L02m2  ,L12m1  ,L12m2  ,L22m1  ,L22m2  ,L0m1 ,L0m2 ,L1m1 ,L1m2 ,L2m1 ,L2m2]);
[cy5,ty5] = coeffs(Y5_TH, [m1,m2,mb,I1,I2,Ix,L0m1,L0m2,L1m1,L1m2,L2m1,L2m2,L02m1,L02m2,L12m1,L12m2,L22m1,L22m2,L0L1m1,L0L1m2,L1L2m1,L1L2m2,L0L2m1,L0L2m2]);
%===================================
Y6_TH=subs(Y6_TH,[L0*L1*m1,L0*L1*m2,L1*L2*m1,L1*L2*m2,L0*L2*m1,L0*L2*m2,L0^2*m1,L0^2*m2,L1^2*m1,L1^2*m2,L2^2*m1,L2^2*m2,L0*m1,L0*m2,L1*m1,L1*m2,L2*m1,L2*m2] ...
,[L0L1m1  ,L0L1m2  ,L1L2m1  ,L1L2m2  ,L0L2m1  ,L0L2m2  ,L02m1  ,L02m2  ,L12m1  ,L12m2  ,L22m1  ,L22m2  ,L0m1 ,L0m2 ,L1m1 ,L1m2 ,L2m1 ,L2m2]);
[cy6,ty6] = coeffs(Y6_TH, [m1,m2,mb,I1,I2,Ix,L0m1,L0m2,L1m1,L1m2,L2m1,L2m2,L02m1,L02m2,L12m1,L12m2,L22m1,L22m2,L0L1m1,L0L1m2,L1L2m1,L1L2m2,L0L2m1,L0L2m2]);
%===================================
Y7_TH=subs(Y7_TH,[L0*L1*m1,L0*L1*m2,L1*L2*m1,L1*L2*m2,L0*L2*m1,L0*L2*m2,L0^2*m1,L0^2*m2,L1^2*m1,L1^2*m2,L2^2*m1,L2^2*m2,L0*m1,L0*m2,L1*m1,L1*m2,L2*m1,L2*m2] ...
,[L0L1m1  ,L0L1m2  ,L1L2m1  ,L1L2m2  ,L0L2m1  ,L0L2m2  ,L02m1  ,L02m2  ,L12m1  ,L12m2  ,L22m1  ,L22m2  ,L0m1 ,L0m2 ,L1m1 ,L1m2 ,L2m1 ,L2m2]);
[cy7,ty7] = coeffs(Y7_TH, [m1,m2,mb,I1,I2,Ix,L0m1,L0m2,L1m1,L1m2,L2m1,L2m2,L02m1,L02m2,L12m1,L12m2,L22m1,L22m2,L0L1m1,L0L1m2,L1L2m1,L1L2m2,L0L2m1,L0L2m2]);
%===================================
Y8_TH=subs(Y8_TH,[L0*L1*m1,L0*L1*m2,L1*L2*m1,L1*L2*m2,L0*L2*m1,L0*L2*m2,L0^2*m1,L0^2*m2,L1^2*m1,L1^2*m2,L2^2*m1,L2^2*m2,L0*m1,L0*m2,L1*m1,L1*m2,L2*m1,L2*m2] ...
,[L0L1m1  ,L0L1m2  ,L1L2m1  ,L1L2m2  ,L0L2m1  ,L0L2m2  ,L02m1  ,L02m2  ,L12m1  ,L12m2  ,L22m1  ,L22m2  ,L0m1 ,L0m2 ,L1m1 ,L1m2 ,L2m1 ,L2m2]);
[cy8,ty8] = coeffs(Y8_TH, [m1,m2,mb,I1,I2,Ix,L0m1,L0m2,L1m1,L1m2,L2m1,L2m2,L02m1,L02m2,L12m1,L12m2,L22m1,L22m2,L0L1m1,L0L1m2,L1L2m1,L1L2m2,L0L2m1,L0L2m2]);

Yi = [cy1;cy2;cy3;cy4;cy5;cy6;cy7;cy8];

%% =================================================================

syms xe ye  ze  phe  the  epe
syms xde  yde  zde  phde  thde  epde
syms Kc1  Mc1  Kc2 Mc2 Kc3 Mc3 Kc4 Mc4 Kc5 Mc5 Kc6 Mc6
Xe=[xe; ye; ze; epe; the; phe];
Xde=[xde; yde; zde; epde; thde; phde];

%% ======= Yl ==============

Fe_reg = [Xe(1),Xde(1),zeros(1,10);
zeros(1,2),Xe(2),Xde(2),zeros(1,8);
zeros(1,4),Xe(3),Xde(3),zeros(1,6);
zeros(1,6),Xe(4),Xde(4),zeros(1,4);
zeros(1,8),Xe(5),Xde(5),zeros(1,2);
zeros(1,10),Xe(6),Xde(6)];

Y_l = JT*Fe_reg;

%% ======= Yw ==============
D_ex_reg1 = [z^2*sin(th), z^2*cos(th), 0, 0];
D_ex_reg2 = [0, 0,z^2*sin(ph), z^2*cos(ph)];
D_ex_reg3 = zeros(1,4);
D_ex_reg4 = zeros(1,4);
D_ex_reg5 = zeros(1,4);
D_ex_reg6 = zeros(1,4);
D_ex_reg7 = zeros(1,4);
D_ex_reg8 = zeros(1,4);
%% ======= Yl ==============
JT_Fe_reg1=[ xe, xde, 0, 0, 0, 0, 0, 0, 0, 0, 0, 0];
JT_Fe_reg2=[ 0, 0, ye, yde, 0, 0, 0, 0, 0, 0, 0, 0];
JT_Fe_reg3=[ 0, 0, 0, 0, ze, zde, 0, 0, 0, 0, 0, 0];
JT_Fe_reg4=[ -xe*((cos(ep)*sin(ph) - cos(ph)*sin(ep)*sin(th))*(L0 + L1*sin(th1) + L2*cos(th2)*sin(th1)) - cos(th1)*(L1 + L2*cos(th2))*(cos(ep)*cos(ph) + sin(ep)*sin(ph)*sin(th)) + L2*cos(th)*sin(ep)*sin(th2)), -xde*((cos(ep)*sin(ph) - cos(ph)*sin(ep)*sin(th))*(L0 + L1*sin(th1) + L2*cos(th2)*sin(th1)) - cos(th1)*(L1 + L2*cos(th2))*(cos(ep)*cos(ph) + sin(ep)*sin(ph)*sin(th)) + L2*cos(th)*sin(ep)*sin(th2)), ye*(cos(th1)*(L1 + L2*cos(th2))*(cos(ph)*sin(ep) - cos(ep)*sin(ph)*sin(th)) - (sin(ep)*sin(ph) + cos(ep)*cos(ph)*sin(th))*(L0 + L1*sin(th1) + L2*cos(th2)*sin(th1)) + L2*cos(ep)*cos(th)*sin(th2)), yde*(cos(th1)*(L1 + L2*cos(th2))*(cos(ph)*sin(ep) - cos(ep)*sin(ph)*sin(th)) - (sin(ep)*sin(ph) + cos(ep)*cos(ph)*sin(th))*(L0 + L1*sin(th1) + L2*cos(th2)*sin(th1)) + L2*cos(ep)*cos(th)*sin(th2)), 0, 0, 0, 0, 0, 0, phe, phde];
JT_Fe_reg5=[ -xe*cos(ep)*(L2*sin(th)*sin(th2) + cos(ph)*cos(th)*(L0 + L1*sin(th1) + L2*cos(th2)*sin(th1)) + cos(th)*cos(th1)*sin(ph)*(L1 + L2*cos(th2))), -xde*cos(ep)*(L2*sin(th)*sin(th2) + cos(ph)*cos(th)*(L0 + L1*sin(th1) + L2*cos(th2)*sin(th1)) + cos(th)*cos(th1)*sin(ph)*(L1 + L2*cos(th2))), -ye*sin(ep)*(L2*sin(th)*sin(th2) + cos(ph)*cos(th)*(L0 + L1*sin(th1) + L2*cos(th2)*sin(th1)) + cos(th)*cos(th1)*sin(ph)*(L1 + L2*cos(th2))), -yde*sin(ep)*(L2*sin(th)*sin(th2) + cos(ph)*cos(th)*(L0 + L1*sin(th1) + L2*cos(th2)*sin(th1)) + cos(th)*cos(th1)*sin(ph)*(L1 + L2*cos(th2))), ze*(L0*cos(ph)*sin(th) - L2*cos(th)*sin(th2) + L1*cos(ph)*sin(th)*sin(th1) + L1*cos(th1)*sin(ph)*sin(th) + L2*cos(ph)*cos(th2)*sin(th)*sin(th1) + L2*cos(th1)*cos(th2)*sin(ph)*sin(th)), zde*(L0*cos(ph)*sin(th) - L2*cos(th)*sin(th2) + L1*cos(ph)*sin(th)*sin(th1) + L1*cos(th1)*sin(ph)*sin(th) + L2*cos(ph)*cos(th2)*sin(th)*sin(th1) + L2*cos(th1)*cos(th2)*sin(ph)*sin(th)), -epe*sin(ep), -epde*sin(ep), the*cos(ep), thde*cos(ep), 0, 0];
JT_Fe_reg6=[ xe*(sin(th)*((cos(ep)*sin(ph) - cos(ph)*sin(ep)*sin(th))*(L0 + L1*sin(th1) + L2*cos(th2)*sin(th1)) - cos(th1)*(L1 + L2*cos(th2))*(cos(ep)*cos(ph) + sin(ep)*sin(ph)*sin(th)) + L2*cos(th)*sin(ep)*sin(th2)) - cos(th)*sin(ep)*(L2*sin(th)*sin(th2) + cos(ph)*cos(th)*(L0 + L1*sin(th1) + L2*cos(th2)*sin(th1)) + cos(th)*cos(th1)*sin(ph)*(L1 + L2*cos(th2)))), xde*(sin(th)*((cos(ep)*sin(ph) - cos(ph)*sin(ep)*sin(th))*(L0 + L1*sin(th1) + L2*cos(th2)*sin(th1)) - cos(th1)*(L1 + L2*cos(th2))*(cos(ep)*cos(ph) + sin(ep)*sin(ph)*sin(th)) + L2*cos(th)*sin(ep)*sin(th2)) - cos(th)*sin(ep)*(L2*sin(th)*sin(th2) + cos(ph)*cos(th)*(L0 + L1*sin(th1) + L2*cos(th2)*sin(th1)) + cos(th)*cos(th1)*sin(ph)*(L1 + L2*cos(th2)))), -ye*(sin(th)*(cos(th1)*(L1 + L2*cos(th2))*(cos(ph)*sin(ep) - cos(ep)*sin(ph)*sin(th)) - (sin(ep)*sin(ph) + cos(ep)*cos(ph)*sin(th))*(L0 + L1*sin(th1) + L2*cos(th2)*sin(th1)) + L2*cos(ep)*cos(th)*sin(th2)) - cos(ep)*cos(th)*(L2*sin(th)*sin(th2) + cos(ph)*cos(th)*(L0 + L1*sin(th1) + L2*cos(th2)*sin(th1)) + cos(th)*cos(th1)*sin(ph)*(L1 + L2*cos(th2)))), -yde*(sin(th)*(cos(th1)*(L1 + L2*cos(th2))*(cos(ph)*sin(ep) - cos(ep)*sin(ph)*sin(th)) - (sin(ep)*sin(ph) + cos(ep)*cos(ph)*sin(th))*(L0 + L1*sin(th1) + L2*cos(th2)*sin(th1)) + L2*cos(ep)*cos(th)*sin(th2)) - cos(ep)*cos(th)*(L2*sin(th)*sin(th2) + cos(ph)*cos(th)*(L0 + L1*sin(th1) + L2*cos(th2)*sin(th1)) + cos(th)*cos(th1)*sin(ph)*(L1 + L2*cos(th2)))), -ze*cos(th)*((L2*cos(ph + th1 - th2))/2 + L1*cos(ph + th1) - L0*sin(ph) + (L2*cos(ph + th1 + th2))/2), -zde*cos(th)*((L2*cos(ph + th1 - th2))/2 + L1*cos(ph + th1) - L0*sin(ph) + (L2*cos(ph + th1 + th2))/2), epe*cos(ep)*cos(th), epde*cos(ep)*cos(th), the*cos(th)*sin(ep), thde*cos(th)*sin(ep), -phe*sin(th), -phde*sin(th)];
JT_Fe_reg7= [ -xe*((L1*sin(th1) + L2*cos(th2)*sin(th1))*(cos(ph)*sin(ep) - cos(ep)*sin(ph)*sin(th)) + (L1*cos(th1) + L2*cos(th1)*cos(th2))*(sin(ep)*sin(ph) + cos(ep)*cos(ph)*sin(th))), -xde*((L1*sin(th1) + L2*cos(th2)*sin(th1))*(cos(ph)*sin(ep) - cos(ep)*sin(ph)*sin(th)) + (L1*cos(th1) + L2*cos(th1)*cos(th2))*(sin(ep)*sin(ph) + cos(ep)*cos(ph)*sin(th))), ye*((L1*sin(th1) + L2*cos(th2)*sin(th1))*(cos(ep)*cos(ph) + sin(ep)*sin(ph)*sin(th)) + (L1*cos(th1) + L2*cos(th1)*cos(th2))*(cos(ep)*sin(ph) - cos(ph)*sin(ep)*sin(th))), yde*((L1*sin(th1) + L2*cos(th2)*sin(th1))*(cos(ep)*cos(ph) + sin(ep)*sin(ph)*sin(th)) + (L1*cos(th1) + L2*cos(th1)*cos(th2))*(cos(ep)*sin(ph) - cos(ph)*sin(ep)*sin(th))), -ze*cos(ph + th1)*cos(th)*(L1 + L2*cos(th2)), -zde*cos(ph + th1)*cos(th)*(L1 + L2*cos(th2)), epe*cos(ep)*cos(th), epde*cos(ep)*cos(th), the*cos(th)*sin(ep), thde*cos(th)*sin(ep), -phe*sin(th), -phde*sin(th)];
JT_Fe_reg8=[ xe*(L2*cos(ep)*cos(th)*cos(th2) - L2*cos(th1)*sin(th2)*(cos(ph)*sin(ep) - cos(ep)*sin(ph)*sin(th)) + L2*sin(th1)*sin(th2)*(sin(ep)*sin(ph) + cos(ep)*cos(ph)*sin(th))), xde*(L2*cos(ep)*cos(th)*cos(th2) - L2*cos(th1)*sin(th2)*(cos(ph)*sin(ep) - cos(ep)*sin(ph)*sin(th)) + L2*sin(th1)*sin(th2)*(sin(ep)*sin(ph) + cos(ep)*cos(ph)*sin(th))), ye*(L2*cos(th)*cos(th2)*sin(ep) + L2*cos(th1)*sin(th2)*(cos(ep)*cos(ph) + sin(ep)*sin(ph)*sin(th)) - L2*sin(th1)*sin(th2)*(cos(ep)*sin(ph) - cos(ph)*sin(ep)*sin(th))), yde*(L2*cos(th)*cos(th2)*sin(ep) + L2*cos(th1)*sin(th2)*(cos(ep)*cos(ph) + sin(ep)*sin(ph)*sin(th)) - L2*sin(th1)*sin(th2)*(cos(ep)*sin(ph) - cos(ph)*sin(ep)*sin(th))), ze*(L2*cos(ph)*cos(th)*sin(th1)*sin(th2) - L2*cos(th2)*sin(th) + L2*cos(th)*cos(th1)*sin(ph)*sin(th2)), zde*(L2*cos(ph)*cos(th)*sin(th1)*sin(th2) - L2*cos(th2)*sin(th) + L2*cos(th)*cos(th1)*sin(ph)*sin(th2)), epe*(cos(th1)*(sin(ep)*sin(ph) + cos(ep)*cos(ph)*sin(th)) + sin(th1)*(cos(ph)*sin(ep) - cos(ep)*sin(ph)*sin(th))), epde*(cos(th1)*(sin(ep)*sin(ph) + cos(ep)*cos(ph)*sin(th)) + sin(th1)*(cos(ph)*sin(ep) - cos(ep)*sin(ph)*sin(th))), -the*(cos(th1)*(cos(ep)*sin(ph) - cos(ph)*sin(ep)*sin(th)) + sin(th1)*(cos(ep)*cos(ph) + sin(ep)*sin(ph)*sin(th))), -thde*(cos(th1)*(cos(ep)*sin(ph) - cos(ph)*sin(ep)*sin(th)) + sin(th1)*(cos(ep)*cos(ph) + sin(ep)*sin(ph)*sin(th))), phe*cos(ph + th1)*cos(th), phde*cos(ph + th1)*cos(th)]; 

%% ==================== Ys ================================= 
Ys=[Ya(1,:),JT_Fe_reg1,D_ex_reg1;
Ya(2,:),JT_Fe_reg2,D_ex_reg2;
Ya(3,:),JT_Fe_reg3,D_ex_reg3;
Ya(4,:),JT_Fe_reg4,D_ex_reg4;
Ya(5,:),JT_Fe_reg5,D_ex_reg5;
Ya(6,:),JT_Fe_reg6,D_ex_reg6;
Ya(7,:),JT_Fe_reg7,D_ex_reg7;
Ya(8,:),JT_Fe_reg8,D_ex_reg8];

%% ==================== hs ==================================
 hs = [m1;m2;mb;I1;I2;Ix;L0*m1;L0*m2;L1*m1;L1*m2;L2*m1;L2*m2;L0^2*m1;L0^2*m2;L1^2*m1;L1^2*m2;L2^2*m

\end{lstlisting}
