# Supplementary material for: Controller Design and Implementation of a New Quadrotor Manipulation System
Source: arXiv:1904.08498 source file (2025-09-04)
Supplement: Supplementary file 3 [file Appendix_laser.tex]

\chapter{Laser Range Finder} \label{app:experimentalsystem-laser}

% change according to folder and file names
\ifpdf
    \graphicspath{{10_Appendices/figures/PNG/}{10_Appendices/figures/PDF/}{10_Appendices/figures/}}
\else
    \graphicspath{{10_Appendices/figures/EPS/}{10_Appendices/figures/}}
\fi

% ----------------------- contents from here ------------------------

URG-04LX is a laser sensor for area scanning, see Fig. \ref{fig:laser_top}. The light source of the sensor is infrared laser of wavelength 785nm with laser class 1 safety. Scan area is $240^{\circ}$  semicircle with maximum radius 4000mm.
Principle of distance measurement is based on calculation of the phase difference, due to which
it is possible to obtain stable measurement with minimum influence from object’s color and reflectance 
\begin{figure}[!h]
	\centering
	\includegraphics[width=0.5\columnwidth]{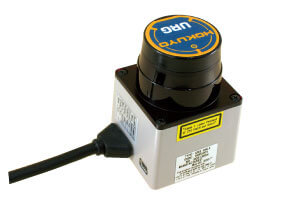}
	\caption{URG-04LX Laser Range Finder \cite{hokuyo}}
	\label{fig:laser_top}
\end{figure}

It has the following features:
\begin{itemize}
	\item High accuracy, high resolution and wide angle which provide the best solution for autonomous robots moving in the unknown environment.
	
	\item Compact size allows more designing freedom. Light weight and low power consumption contribute to the long time operations.
	
	\item No influence by how bright the environment will be. Excellent performance in darkness.
	Recognizing human body's size and position without hurting their privacy.
\end{itemize}
Fig. \ref{fig:laser_dect} illustrates the principle of operation of the URG-04LX. The laser emits an infrared beam, and a rotating mirror changes the beam’s direction. Then the laser
hits the surface of an object and is reflected. The direction of reflected light is changed again by a rotating mirror, and captured by the photo diode. The phases of the emitted and received light are compared and the distance between the sensor and the object is calculated. A rotating mirror sweeps the laser beam horizontally over a range of $240^{\circ}$, with an angular resolution of $0.36^{\circ}$. As the mirror rotates at about 600 rpm, the scan rate is about 100 msec. 

\begin{figure}[!h]
	\centering
	\includegraphics[width=0.8\columnwidth]{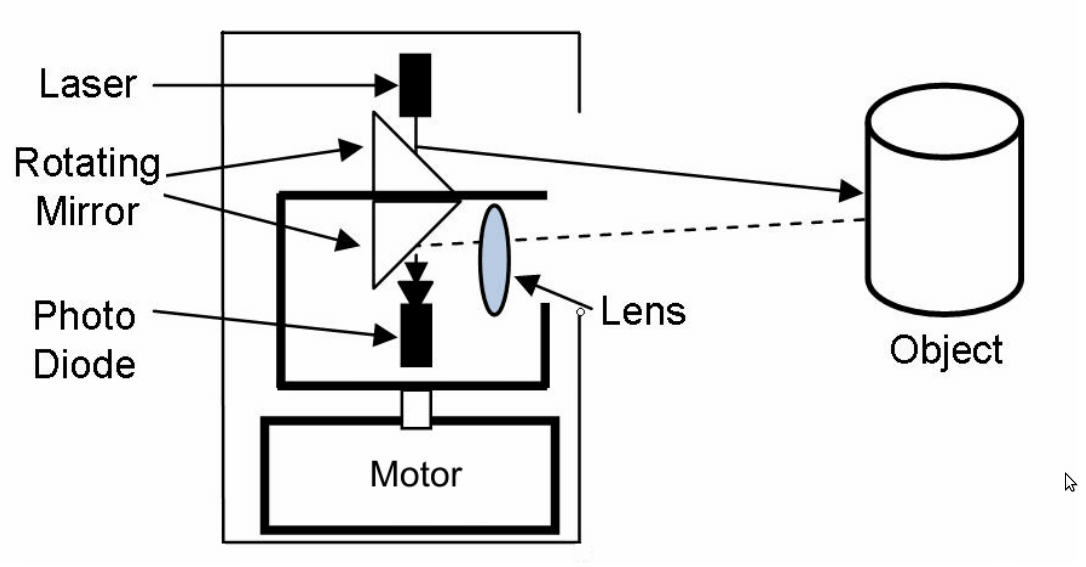}
	\caption{The principle of operation of the URG-04LX \cite{okubo2009characterization}}
	\label{fig:laser_dect}
\end{figure}
%===========================================================
Technical specifications of this device is given in Table \ref{tab:laser_spec}.

\begin{table}[!h]
	\caption{Laser Range Finder, URG-04LX, specifications \cite{hokuyo ,okubo2009characterization}}
	\label{tab:laser_spec}
	\begin{center}
		\begin{tabu}{|X|X|}
			\hline
			Model No. & URG-04LX\\
			\hline
			Power source  & 5VDC$\pm$5\%. Sensor will not operate with USB bus power. Prepare power source separately.
			\\
			\hline
			Current consumption & 500mA or less(800mA when start-up)\\
			\hline
			Measuring area & 60 to 4095mm(white paper with 70mm) $240^{\circ}$\\
			\hline
			Accuracy &  is $\pm$ 10 mm for distances of less than 1 m. For greater distances, the
			error is quoted as $\pm$2\%  \\
			\hline
			Repeatability & 60 to 1,000mm : $\pm$ 10mm \\
			\hline
			Angular resolution &  Step angle : approx. 0.36°(360°/1,024 steps) \\
			\hline
			Light source & Semiconductor laser diode (wave length =785nm) \\
			\hline
			Scanning time & 100ms/scan\\
			\hline
			Noise & 25dB or less\\
			\hline
			Interface & USB, RS-232C(19.2k, 57.6k, 115.2k, 250k, 500k, 750kbps)\\
			\hline
			Ambient temperature/humidity &  -10 to +50 degrees C, 85\% or less(Not condensing, not icing)\\
			\hline
			Vibration resistance & 10 to 55Hz, double amplitude 1.5mm Each 2 hour in X, Y and Z directions\\
			\hline
			Impact resistance & 196m/$s^2$, Each 10 time in X, Y and Z directions\\
			\hline
			Weight & Approx. 160g\\
			\hline
			Accessory & Cable for power communication/input-output(1.5m),
			D-sub connector with 9 pins\\
			\hline
		\end{tabu}
	\end{center}
\end{table}

%==============================================

Fig. \ref{fig:laser_dim} illustrates schematic diagrams with the relevant dimensions.
\begin{figure}[!h]
	\centering
	\includegraphics[width=0.8\columnwidth]{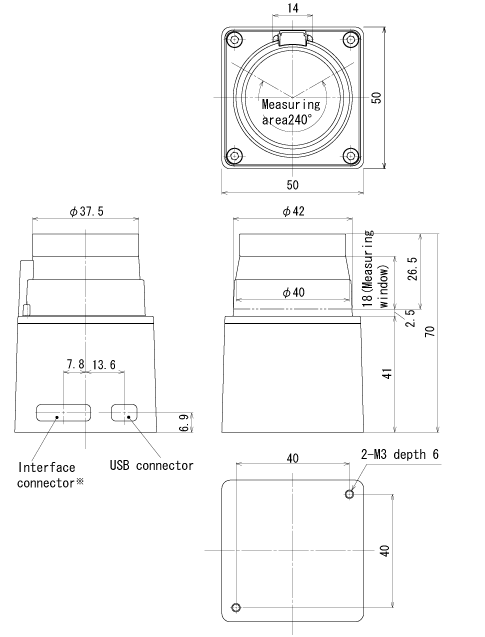}
	\caption{External dimension of the Laser Range Finder URG-04LX \cite{hokuyo}}
	\label{fig:laser_dim}
\end{figure}

There are two connectors RS-connector (Table \ref{tab:laser_conc}) and USB connector (Table \ref{tab:laser_conc2})
\begin{table}[!h]
	\caption{Laser Range Finder, URG-04LX, Pins of the interface connector \cite{hokuyo}}
	\label{tab:laser_conc}
	\begin{center}
		\begin{tabu}{|X|X|X|}
			\hline
Pin No. & Signals & Colors \\
\hline
1 & N.C. & Red \\
\hline
2 & N.C. & White \\
\hline
3 & OUTPUT(Synchronous output) & Black \\
\hline
4 & GND(5th pin of 9-pin, D-sub connector) & Purple \\
\hline
5 & RxD(3rd pin of 9-pin, D-sub connector) & Yellow \\
\hline
6 & TxD(2nd pin of 9-pin, D-sub connector) & Green \\
\hline
7 & 0V & Blue\\
\hline
8 & DC5V & Brown\\

			\hline
		\end{tabu}
	\end{center}
\end{table}

\begin{table}[!h]
	\caption{Laser Range Finder, URG-04LX, the USB connector}
	\label{tab:laser_conc2}
	\begin{center}
		\begin{tabu}{|X|X|}
			\hline
			Connector Type & USB-miniB (5pin) \\
			\hline
		\end{tabu}
	\end{center}
\end{table}
