# Supplementary material for: Controller Design and Implementation of a New Quadrotor Manipulation System
Source: arXiv:1904.08498 source file (2025-09-04)
Supplement: Supplementary file 4 [file Appendix_manp.tex]

\chapter{Robotic Arm} \label{app:experimentalsystem-manp}
% change according to folder and file names
\ifpdf
\graphicspath{{10_Appendices/figures/PNG/}{10_Appendices/figures/PDF/}{10_Appendices/figures/}}
\else
\graphicspath{{10_Appendices/figures/EPS/}{10_Appendices/figures/}}
\fi

% ----------------------- contents from here ------------------------

Starting with design of the gripper mechanism, a little gripper (Fig. \ref{fig:gripper}), from \uppercase{"lynxmotion"}, is used. It is made from injection molded ABS. This gripper can open to 3.3 cm. It has a driving motor ($mtr_2$), see Fig. \ref{fig:2d_manp_motorsel}, of type servo motor HS-422. This gripper can carry a payload of 200 g \cite{gripper_payload}.
% Thus, a payload of 150 g is chosen as a maximum allowable value for the payload carried by the gripper (for safety purpose).
% ===========================================
\begin{figure}[!h]
	\centering 
	\includegraphics[width=0.5\textwidth]{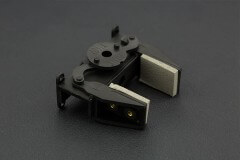}
	\caption{Lightweight gripper \cite{lynxmotion}}
	\label{fig:gripper}
\end{figure}
% ===========================================
% ===========================================
\begin{figure}[!h]
	\centering 
	\includegraphics[width=0.8\textwidth]{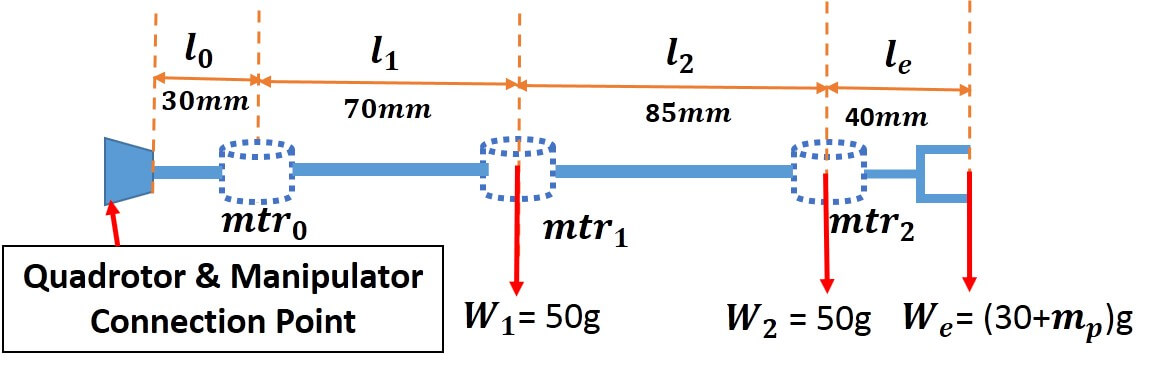}
	\caption{Schematic diagram of the manipulator used to select the joints' motors}
	\label{fig:2d_manp_motorsel}
\end{figure}
% ===========================================

The total length of the arm is chosen such that it can provide enough work space. If the length is increased , then a motor with larger output torque is required, and thus larger weight and more consumed power are resulted.

Based on this design, the required specifications of the selected joints motors are set from Fig. \ref{fig:2d_manp_motorsel}.

The torques, $T_{mtr_0}$ and $T_{mtr_1}$, of motors, $mtr_0$, and $mtr_1$), respectively, see Fig. \ref{fig:2d_manp_motorsel}, can be calculated from(\ref{torque_mtr0} and \ref{torque_mtr1}):
\begin{equation}
T_{mtr_0} = l_1 W_1 + (l_1 + l_2 ) W_2 + (l_1 + l_2 + l_e) W_e
\label{torque_mtr0}
\end{equation}
\begin{equation}
T_{mtr_1} = l_2 W_2 + (l_2 + l_e) W_e
\label{torque_mtr1}
\end{equation}

where $W_e$ is the weight from the end effector and the payload that it has mass of $m_p$.

The average weight of the available motors in the light categories is 50 g (including the arm accessories that will be described next).

Therefore, from the values of lengths and masses shown in Fig. \ref{fig:2d_manp_motorsel}, the value of $T_{mtr_0}$ is 0.45 N.m and $T_{mtr_1}$ is 0.26 N.m (@ payload $m_p$ = 200 g). Multiplying this value by factor of 1.2 for safety, the selected motors should have output torque at least of 0.55 N.m for $mtr_0$ and 0.31 N.m for $mtr_1$.

A digital standard servo (HS-5485HB), see Fig. \ref{fig:servomotor}, is used to provide the rotational motion (Revolute Joint) for joint 1. It has a rotational range of $180^{o}$, weight of 45 g, speed of $350^{o}/s$, and operating voltage of 6 V with maximum running current of 1 A. It is capable of producing a torque of 0.63 N.m. Another  digital standard servo (HS-422) is used for both joint 2 and the gripper. It has a rotational range of 180$^{\circ}$, weight of 45 g, speed of 350$^{\circ}$/s, operating voltage of 6 V with maximum running current of 0.51 A, and torque of 0.32 N.m \cite{lynxmotion}. Figs. \ref{fig:joint1_mtr_dim} and \ref{fig:joint2_mtr_dim} present the dimensions of motors 1 and 2 respectively.
% ===========================================
\begin{figure}[!h]
	\centering
	\includegraphics[width=0.3\columnwidth, height=4cm]{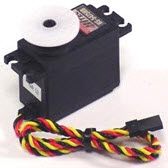}
	\caption{HS-5485HB digital servo motor \cite{lynxmotion}}
	\label{fig:servomotor}
\end{figure}
% ===========================================

% ===========================================
\begin{figure}[!h]
	\centering
	\includegraphics[width=0.3\columnwidth]{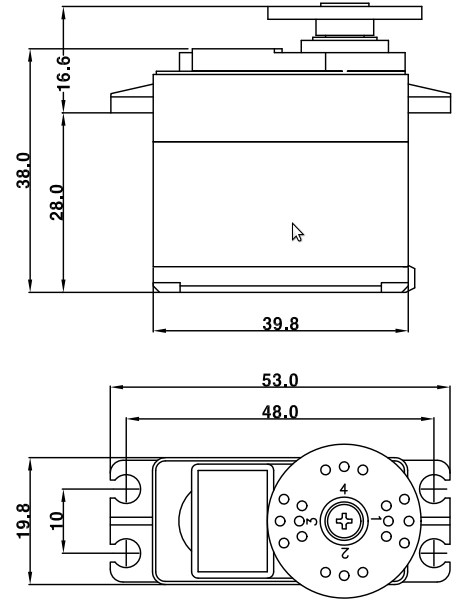}
	\caption{HS-5485HB dimensions \cite{lynxmotion}}
	\label{fig:joint1_mtr_dim}
\end{figure}
% ===========================================
% ===========================================
\begin{figure}[!h]
	\centering
	\includegraphics[width=0.3\columnwidth]{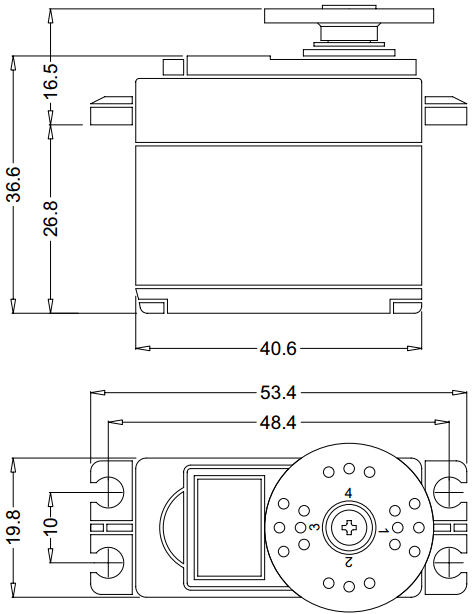}
	\caption{HS-422 dimensions \cite{lynxmotion}}
	\label{fig:joint2_mtr_dim}
\end{figure}
% ===========================================

Fig. \ref{fig:accessories} presents the required accessories to build the the two arms of the manipulator. Also, the dimensions of these accessories are given in Fig. \ref{fig:accessories_dim}.
\begin{figure}[!h]
	\centering
	\begin{tabular}{cc}
		\subfloat[Aluminum Tubing - 1.50 in]{\includegraphics[width=0.4\columnwidth,height=6cm]{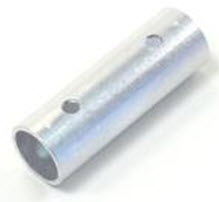}}&
		\subfloat[Aluminum Multi-Purpose Servo Bracket Two Pack]{\includegraphics[width=0.5\columnwidth,height=6cm]{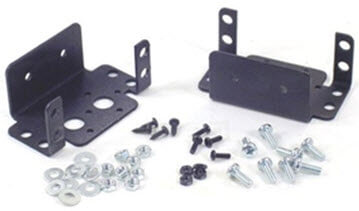}}\\
		\subfloat[Aluminum Tubing Connector Hub]{\includegraphics[width=0.4\columnwidth,height=6cm]{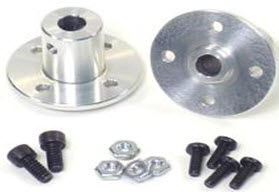}}&
		\subfloat[Aluminum Long "C" Servo Bracket with Ball Bearings Two Pack]{\includegraphics[width=0.5\columnwidth,height=6cm]{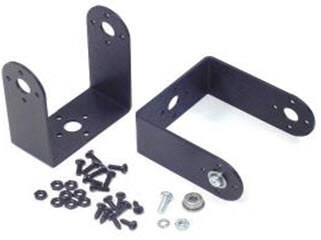}}\\
	\end{tabular}
	\caption{Accessories for building the manipulator: a) Aluminum Tubing, b) Servo Bracket, c) Connector Hub, and d) Long "C" Servo Bracket \cite{lynxmotion}}
	\label{fig:accessories}
\end{figure}
% ===========================================
\begin{figure}[!h]
	\centering
	\begin{tabular}{cc}
		\subfloat[Aluminum Tubing]{\includegraphics[width=0.5\columnwidth,height=7cm]{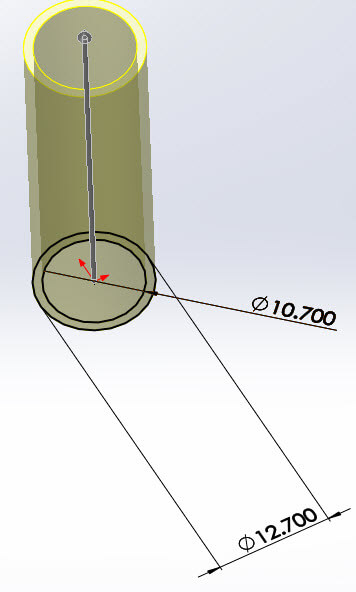}}&
		\subfloat[Servo Bracket]{\includegraphics[width=0.5\columnwidth,height=7cm]{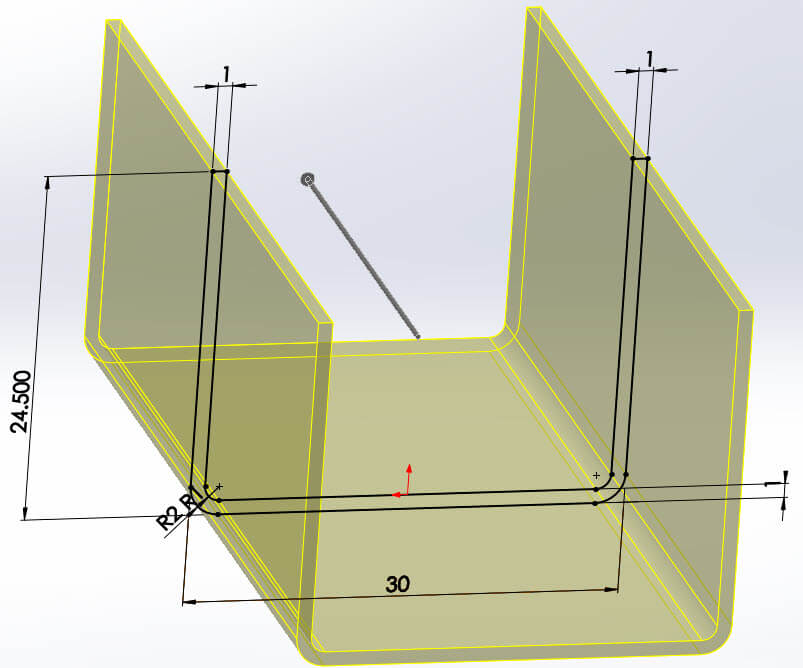}} \\
		\subfloat[Connector Hub]{\includegraphics[width=0.5\columnwidth,height=7cm]{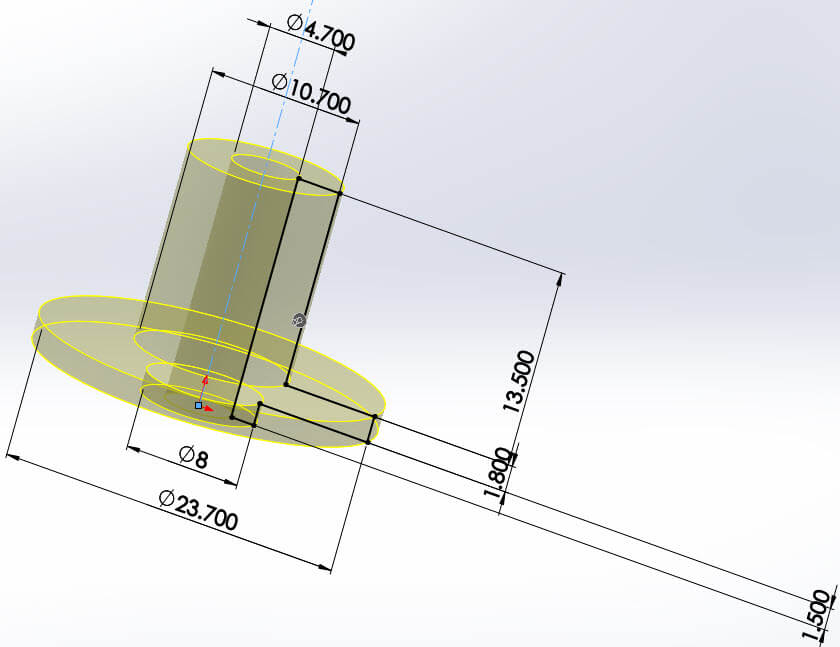}}&
		\subfloat[Aluminum Long "C" Servo Bracket]{\includegraphics[width=0.5\columnwidth,height=7cm]{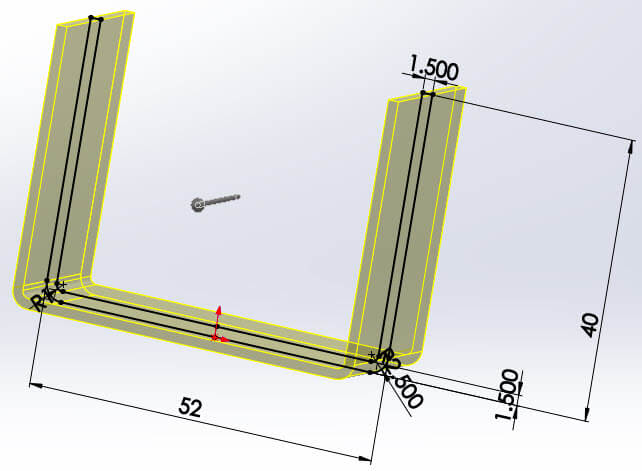}}\\
	\end{tabular}
	\caption{Dimensions of the accessories for building the manipulator in (mm): a) Aluminum Tubing, b) Servo Bracket, c) Connector Hub, and d) Long "C" Servo Bracket.}
	\label{fig:accessories_dim}
\end{figure}
% ===========================================
Serial servo controller (SSC-32) from \uppercase{Lynxmotion}, see Fig. \ref{fig:servocontroller}, is a small preassembled servo controller with some big features. It has high resolution (1 $\mu$s) for accurate positioning, and extremely smooth moves. The range is 0.50 ms to 2.50 ms for a range of about $180^{circ}$. This board contains a MCU of Atmel ATMEGA168-20PU as well as driver interface between the controller unit and the motors. This driver unit operates at voltage of 12 V \cite{lynxmotion}. This unit will take its commands from the Arduino MEGA 2560 board.
\begin{figure}[!h]
	\centering
	\includegraphics[width=0.5\columnwidth]{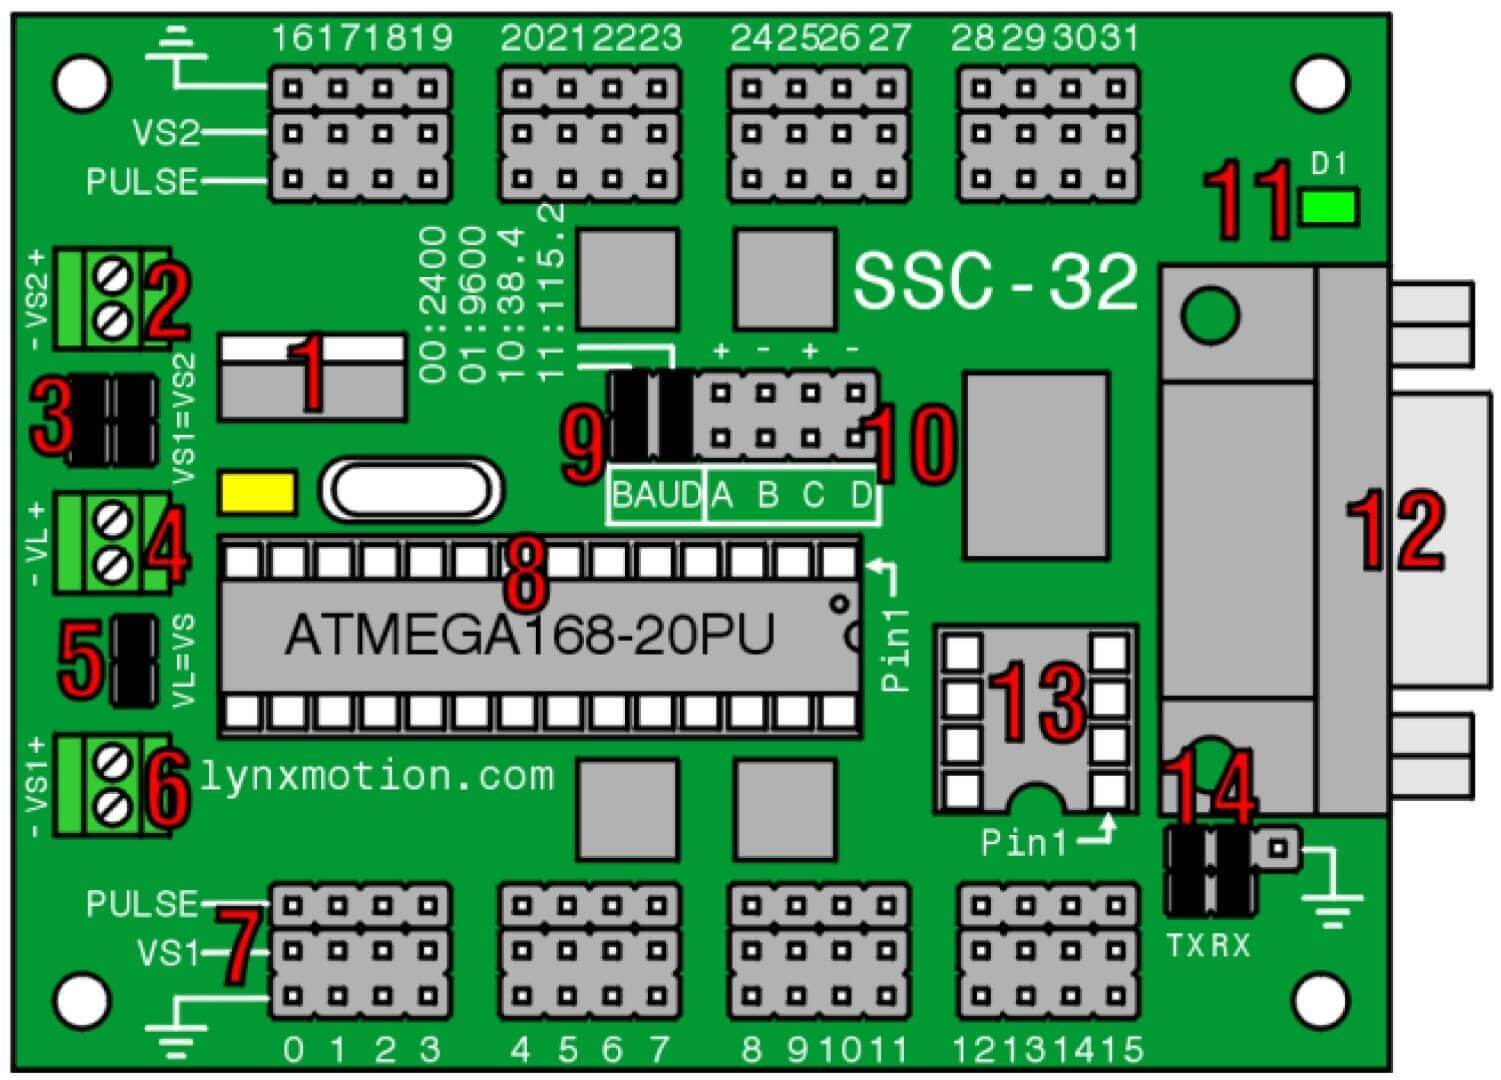}
	\caption{SSC-32 servo controller \cite{lynxmotion}}
	\label{fig:servocontroller}
\end{figure}
% ===========================================
The pin configuration of this board is as following.
\begin{enumerate}
  \item The Low Dropout regulator will provide 5vdc out with as little as 5.5vdc coming in. This is important when
  operating your robot from a battery. It can accept a maximum of 9vdc in. The regulator is rated for 500mA, but we
  are de-rating it to 250mA to prevent the regulator from getting too hot.
  
  \item This terminal connects power to servo channels 16 through 31. Apply 4.8vdc to 6.0vdc for most analog or digital
  servos. This can be directly from a 5-cell NiMH battery pack. 7.2vdc - 7.4vdc can be applied to HSR-5980 or HSR-
  5990 servos. This can be directly from a 6-cell NiMH battery pack or a 2-cell LiPo battery pack. 
  
  \item  These jumpers are used to connect VS1 to VS2. Use this option when you are powering all servos from the same
  battery. Use both jumpers. Alternately, if you want to use two separate battery packs, one on each side, then
  remove both of these jumpers.
  
  \item This is the Logic Voltage, or VL. This input is normally used with a 9vdc battery connector to provide power to the
  ICs and anything connected to the 5vdc lines on the board. The valid range for this terminal is 6vdc - 9vdc. This
  input is used to isolate the logic from the Servo Power Input. It is necessary to remove the VS1=VL jumper when
  powering the servos separately from the logic VL. The SSC-32 should draw 35mA with nothing connected to the
  5vdc output
  
  \item This jumper allows powering the microcontroller and support circuitry from the servo power supply. This requires
  at least 6vdc to operate correctly. If the microcontroller resets when too many servos are moving at the same
  time, it may be necessary to power the microcontroller separately using the VL input. A 9vdc works nicely for this.
  This jumper must be removed when powering the microcontroller separately
  
  \item This terminal connects power to servo channels 16 through 31. Apply 4.8vdc to 6.0vdc for most analog or digital servos. This can be directly from a 5-cell NiMH battery pack. 7.2vdc - 7.4vdc can be applied to HSR-5980 or HSR-
  5990 servos. This can be directly from a 6-cell NiMH battery pack or a 2-cell LiPo battery pack.
  
  \item This is where you connect the servos or other output devices. Use caution and remove power when connecting
  anything to the I/O bus.
  
  \item  This is where the Atmel IC chip goes. Be careful to insert it with Pin 1 in the upper right corner as pictured. Take
  care to not bend the pins.
  
  \item The two BAUD inputs allow configuring the baud rate.
  
  \item The ABCD inputs have both static and latching support. The inputs have internal weak (50k) pullups that are
  used when a Read Digital Input command is used. A normally open switch connected from the input to ground will
  work fine.
  
  \item This is the Processor Good LED. It will light steady when power is applied and will remain lit until the processor
  has received a valid serial command. It will then go out and will blink whenever it is receiving serial data.
  
   \item  Simply plug a straight-through M/F DB9 cable from this plug to a free 9-pin serial port con your PC for receiving
   servo positioning data. Alternately a USB-to-serial adapter will work well. Note, many USB-to-serial adapters
   require a separate power supply to work well.
   \item This is an 8-pin EEPROM socket. 
   \item  This is the TTL serial port or DB9 serial port enable. Install two jumpers as illustrated below to enable the DB9
   port. Install wire connectors to utilize TTL serial communication from a host microcontroller.
\end{enumerate}
Fig. \ref{fig:ssc_jump_serial} presents the way to mount the jumpers of the SSC32 board to enable the communication between this board and the Arduino board such that one can send the motor commands from the Arduino to the SSC32 board. 
% ===========================================
\begin{figure}[!h]
	\centering
	\includegraphics[width=0.5\columnwidth]{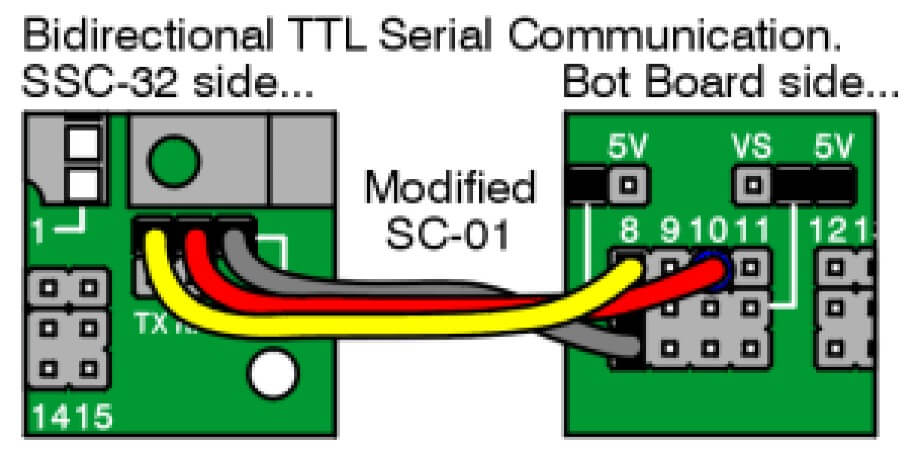}
	\caption{SSC32 board: Shorting bar jumpers to enable serial communication with the Arduino board}
	\label{fig:ssc_jump_serial}
\end{figure}
% ===========================================
One microcontroller that has gotten special attention from the robotics community world-wide is the Arduino.  This microcontroller platform is quite inexpensive and has a C-based language development environment that is very intuitive to use.  From the different versions of the Arduino, the selected one for this project was the Arduino Mega 2560 (see Fig. \ref{fig:arduino2560}). It has 54 digital input/output pins of which 15 can be used as PWM outputs, 16 analog inputs, 4 UARTs (hardware serial ports), 16 MHz crystal oscillator, USB connection, power jack, and 256 KB flash memory for storing code \cite{arduino}. This board has a open source ROS library.
% ===========================================
\begin{figure}[!h]
	\centering
	\includegraphics[width=0.8\columnwidth]{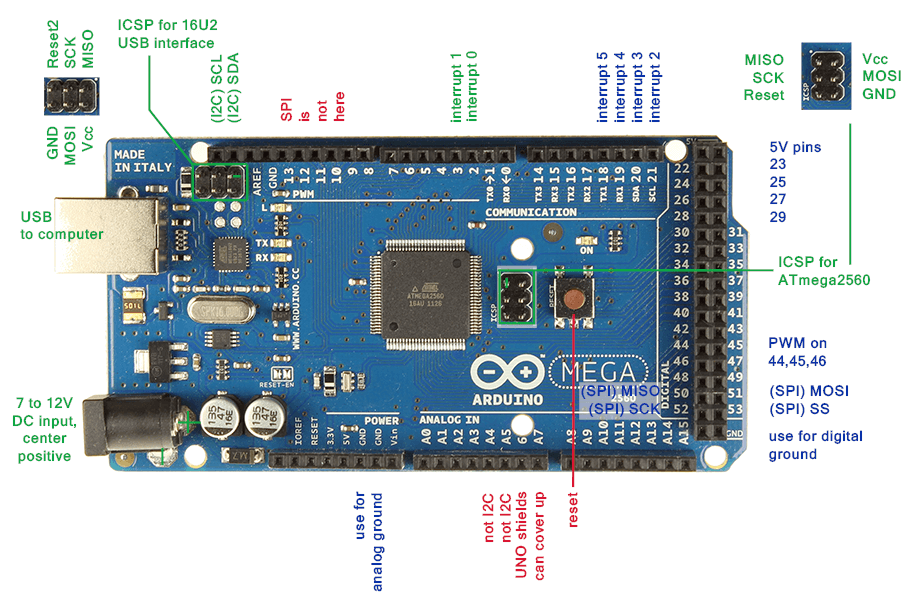}
	\caption{Arduino Mega 2560 board \cite{arduino}}
	\label{fig:arduino2560}
\end{figure}
% ===========================================

Fig. \ref{fig:dc-dc_conv}) shows the circuit diagram for the 12 V to 5V 1.5 A DC-DC converter that is used to power the manipulator's motors. This circuit uses the 7805 IC to converts the 12 VDC from the quadrotor battery to the required 5 VDC at 1.5 A.
% ===========================================
\begin{figure}[!h]
	\centering
	\includegraphics[width=0.8\columnwidth]{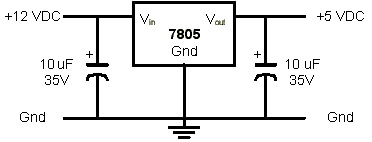}
	\caption{12 V to 5 V 1.5 A DC-DC converter circuit diagram \cite{dc-dc_conv_ref}}
	\label{fig:dc-dc_conv}
\end{figure}
% ===========================================
