# Supplementary material for: Controller Design and Implementation of a New Quadrotor Manipulation System
Source: arXiv:1904.08498 source file (2025-09-04)
Supplement: Supplementary file 5 [file Appendix_quad.tex]

\chapter{Quadrotor Platform} \label{app:experimentalsystem-quad}

% change according to folder and file names
\ifpdf
    \graphicspath{{10_Appendices/figures/PNG/}{10_Appendices/figures/PDF/}{10_Appendices/figures/}}
\else
    \graphicspath{{10_Appendices/figures/EPS/}{10_Appendices/figures/}}
\fi
% ----------------------- contents from here ------------------------

We use a quadrotor from Ascending Technologies (AscTec) of type Pelican that is shown in Fig. \ref{fig:Pelican}
\begin{figure}[!h]
	\centering
	\includegraphics[width=0.9\columnwidth]{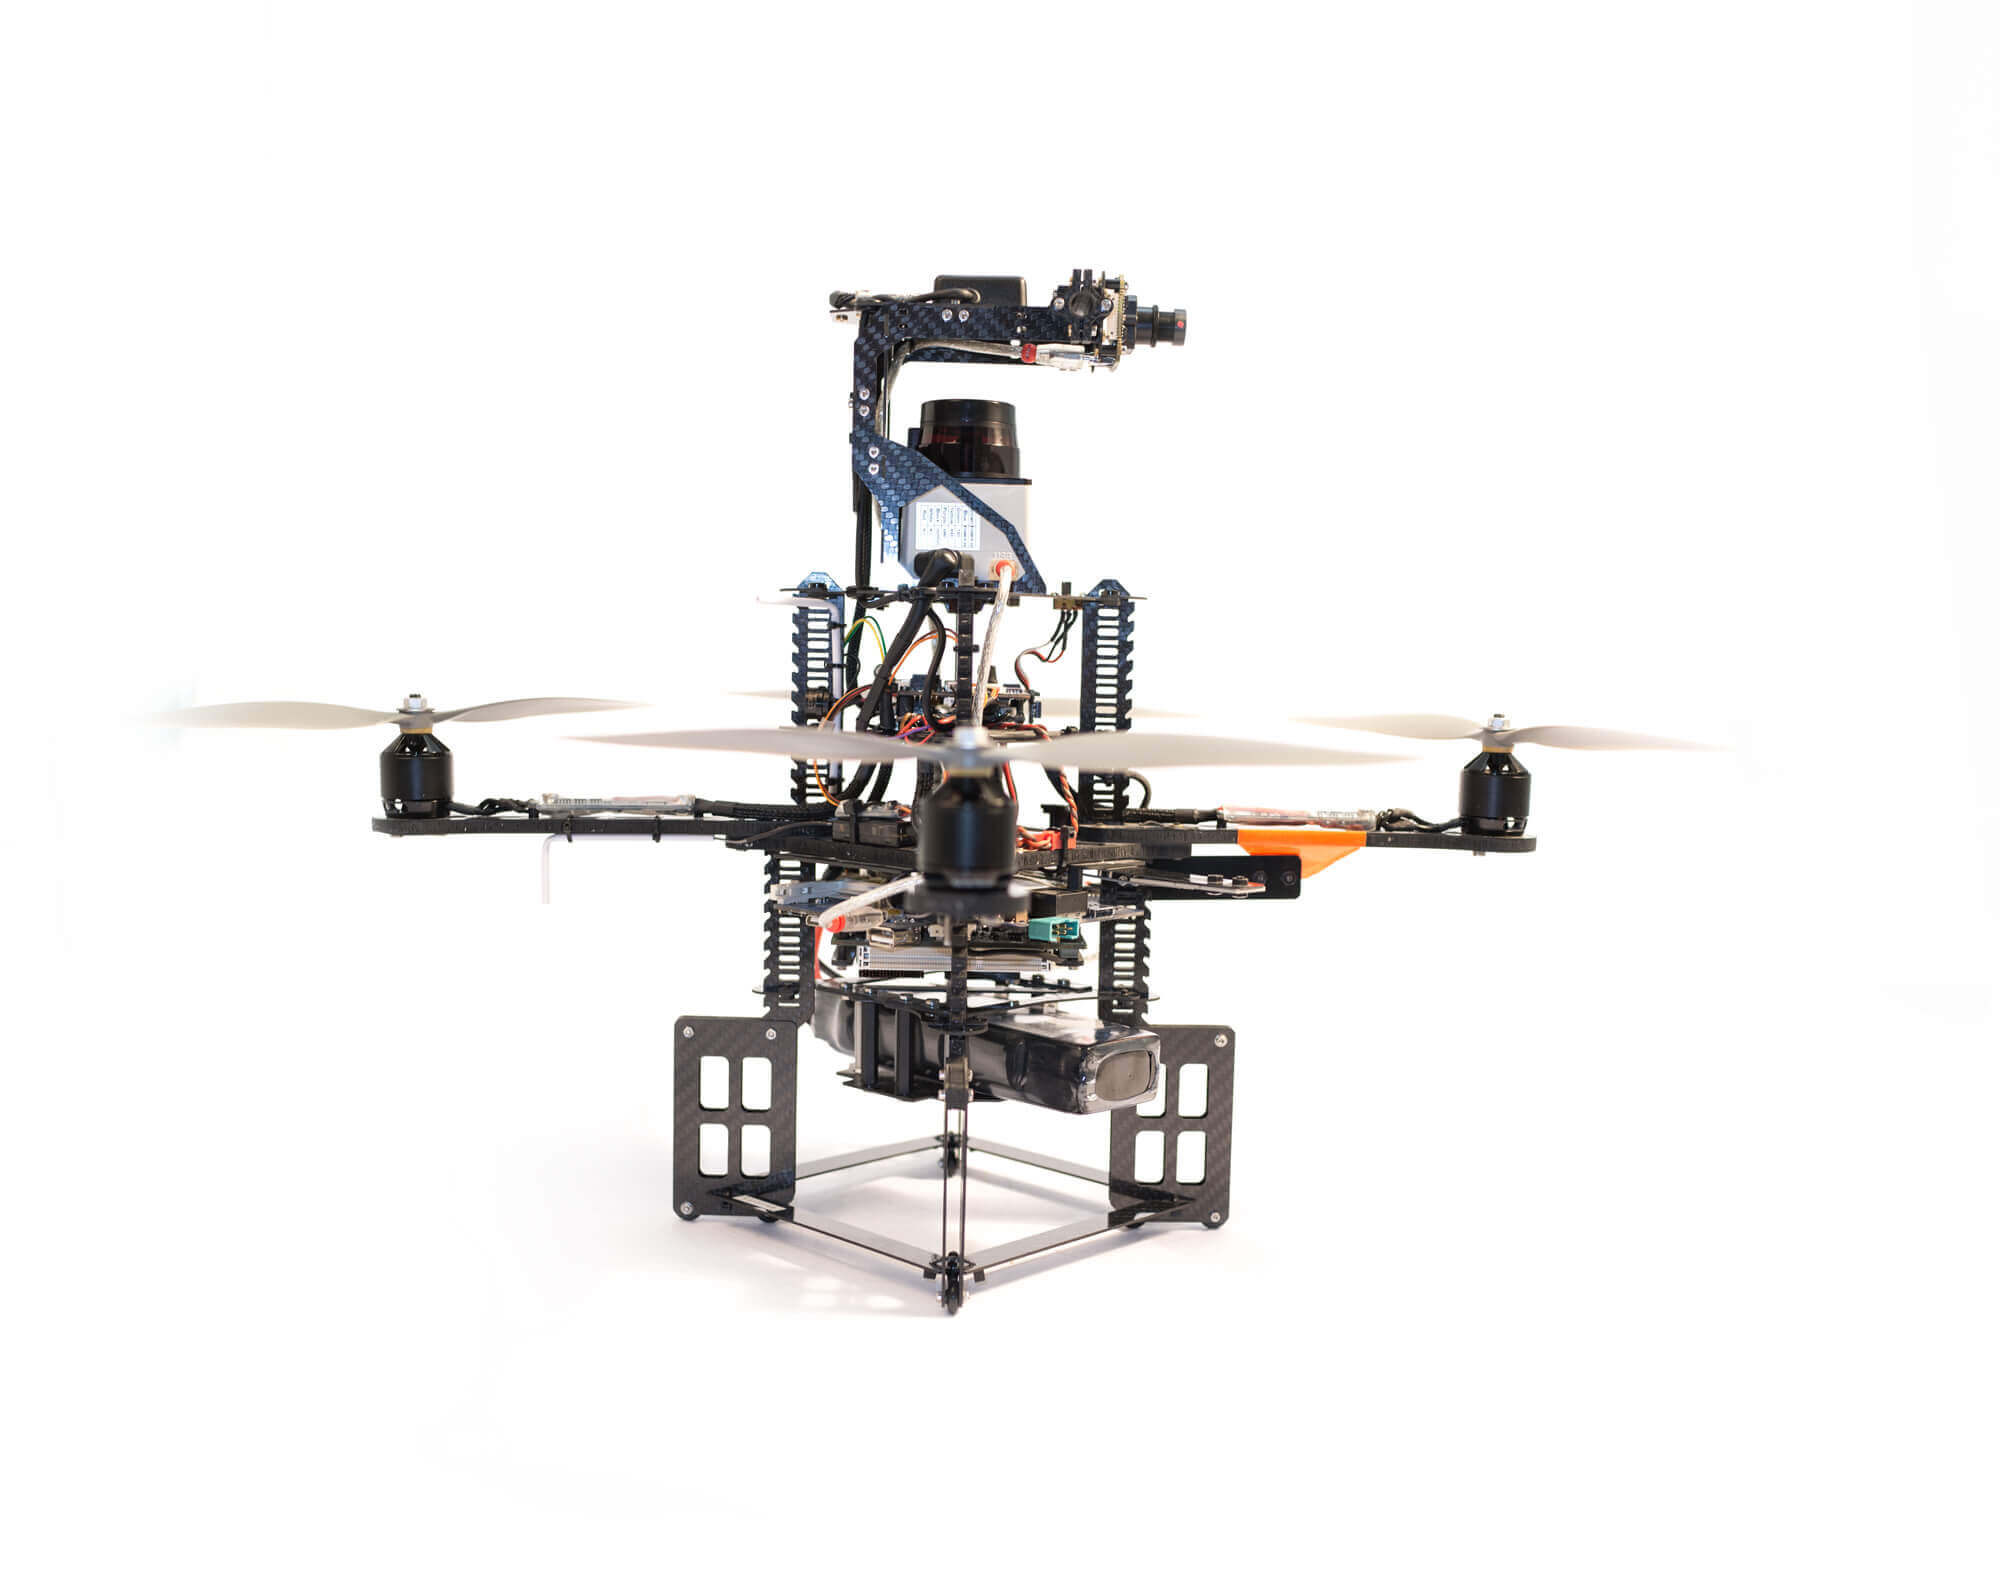}
	\caption{AscTec Pelican quadrotor with full options \cite{asctec}}
	\label{fig:Pelican}
\end{figure}

The propellers are mounted as shown in Fig. \ref{fig:Propeller-turning-directions_Quad}
\begin{figure}[!h]
	\centering
	\includegraphics[width=0.5\columnwidth]{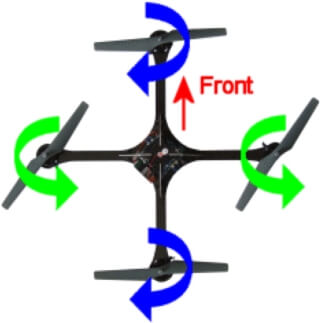}
	\caption{Mounting the propellers \cite{asctec}}
	\label{fig:Propeller-turning-directions_Quad}
\end{figure}

Table \ref{tab:asctec_spec} presents the technical specification for Pelican quadrotor from AscTec. 
% $\SI{10}{kg m s^{-2}}$
\begin{table}[!h]
	\caption{AscTec Pelican, technical Data \cite{asctec}}
	\label{tab:asctec_spec}
	\begin{center}
		\begin{tabu}{|X|X|}
			\hline
Dimensions & 65.1 $\times$ 65.1 $\times$ 18.8 cm \\
		\hline
Propeller size & 10 inch\\
		\hline
Motors & 4 $\times$ 160 W electrical, brushless (sensorless) \\
		\hline
Max. thrust & 36 N\\
		\hline
Max. payload & 650 g\\
		\hline
Max. total weight & 1650 g\\
		\hline
Max. airspeed & 16 m/s\\
		\hline
Max. flight time & 30 mins (without payload)\\
\hline
Range & $\SI{1}{k m}$\\
		\hline
Battery & 6250 mAh (LiPo)\\
			\hline
		\end{tabu}
	\end{center}
\end{table}

The quadrotor dimensions are given in Fig. \ref{fig:pelican_dim}
\begin{figure}[!h]
	\centering
	\includegraphics[width=0.8\columnwidth]{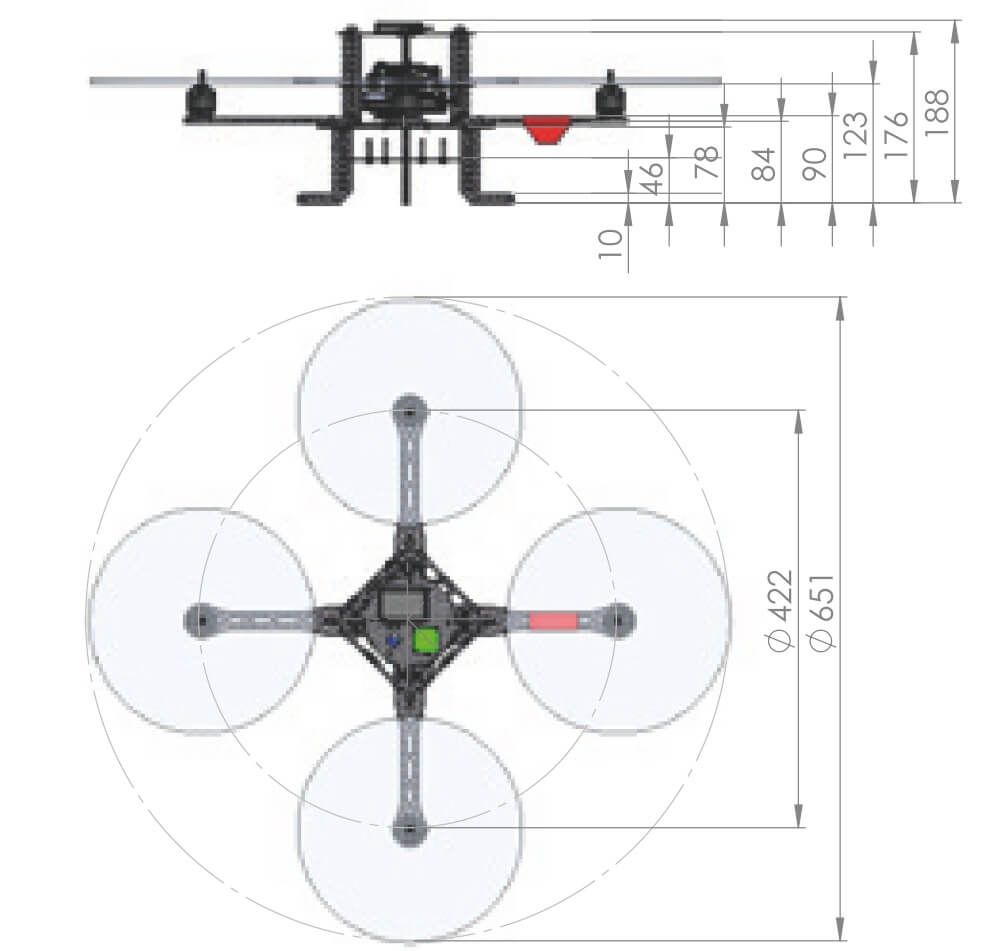}
	\caption{Dimensions of the Pelican quadrotor \cite{asctec}}
	\label{fig:pelican_dim}
\end{figure}

Fig. \ref{fig:auto_view} illustrates functional block diagram of the FCU. This flight control unit contains all necessary sensors to function as an IMU, it also has two onboard ARM7 microprocessors and various communication interfaces.
\begin{figure}[!h]
	\centering
	\includegraphics[width=0.9\columnwidth]{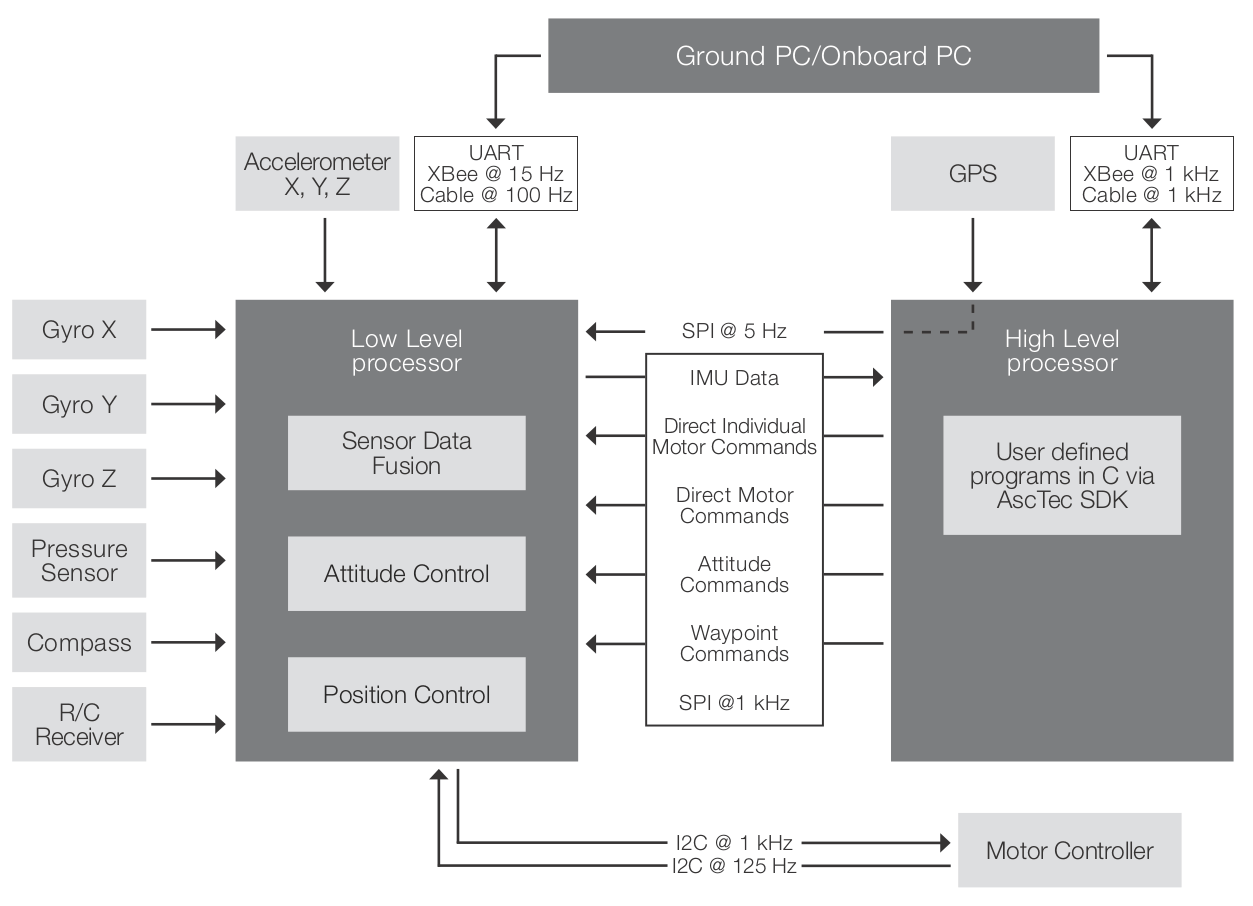}
	\caption{AscTec AutoPilot functional block diagram \cite{asctec}}
	\label{fig:auto_view}
\end{figure}

 It can directly interpret the R/C data sent by the pilot (R/C) and the serial data sent from the ground PC. For automatic missions, you can program and upload our control algorithms directly onto the High Level processor of the UAV.
 
 The LLP handles sensor data processing, data fusion as well as our fast and stable attitude control algorithm with an update rate of 1000 Hz. It also processes the position control algorithm, using the onboard magnetometer and GPS module as additional sensor inputs. Sensor data can be retrieved from the LLP via a serial interface using a predefined serial protocol. Furthermore, the serial interface can be used to send attitude commands (pitch angle, roll angle, yaw rate and thrust) or even waypoint commands to the vehicle depending on the flight mode. The data structures from and to the LLP are
 \begin{itemize}
 	\item LLP STATUS: Status information of the low level processor.
 	\item IMU RAWDATA: Sensor raw-values.
 	\item IMU CALCDATA: Calibrated sensor outputs and data fusion results.
 	\item CTRL OUT: Controller outputs.
 	\item RC Data: Data received by the R/C receiver.
 	\item GPS Data: GPS data.
 	\item GPS Data Advanced: GPS data + position and speed estimates after data fusion.
 \end{itemize}

The HLP can be flashed with a custom algorithm and let it control the flight system. To recover from critical flight situations during the test flights, the pilot can always switch back to the well proven control algorithms on the LLP as a safety backup.

The two microprocessors communicate with an extremely fast rate of 1000 Hz, hence all sensor data is available to the HLP as well. Control commands can be sent back to the LLP at the same frequency, for example the: rotational speed commands for each individual motor, pitch/roll/yaw/thrust commands, attitude commands or waypoint commands. The HLP offers UART (Universal Asynchronous Receiver Transmitter), SPI (Serial Peripheral Interface) and I2C (Inter-Integrated Circuit) interfaces as well as simple port I/Os to connect other devices like additional sensors, servo motors or extension boards. Also custom payloads, can be powered by a 5 V or 12 V supply of the AscTec AutoPilot.

Fig. \ref{fig:AutoPilotV2Desc} shows the pinout and connections of the AscTec AutoPilot board.
\begin{figure}[!h]
	\centering
	\includegraphics[width=0.9\columnwidth]{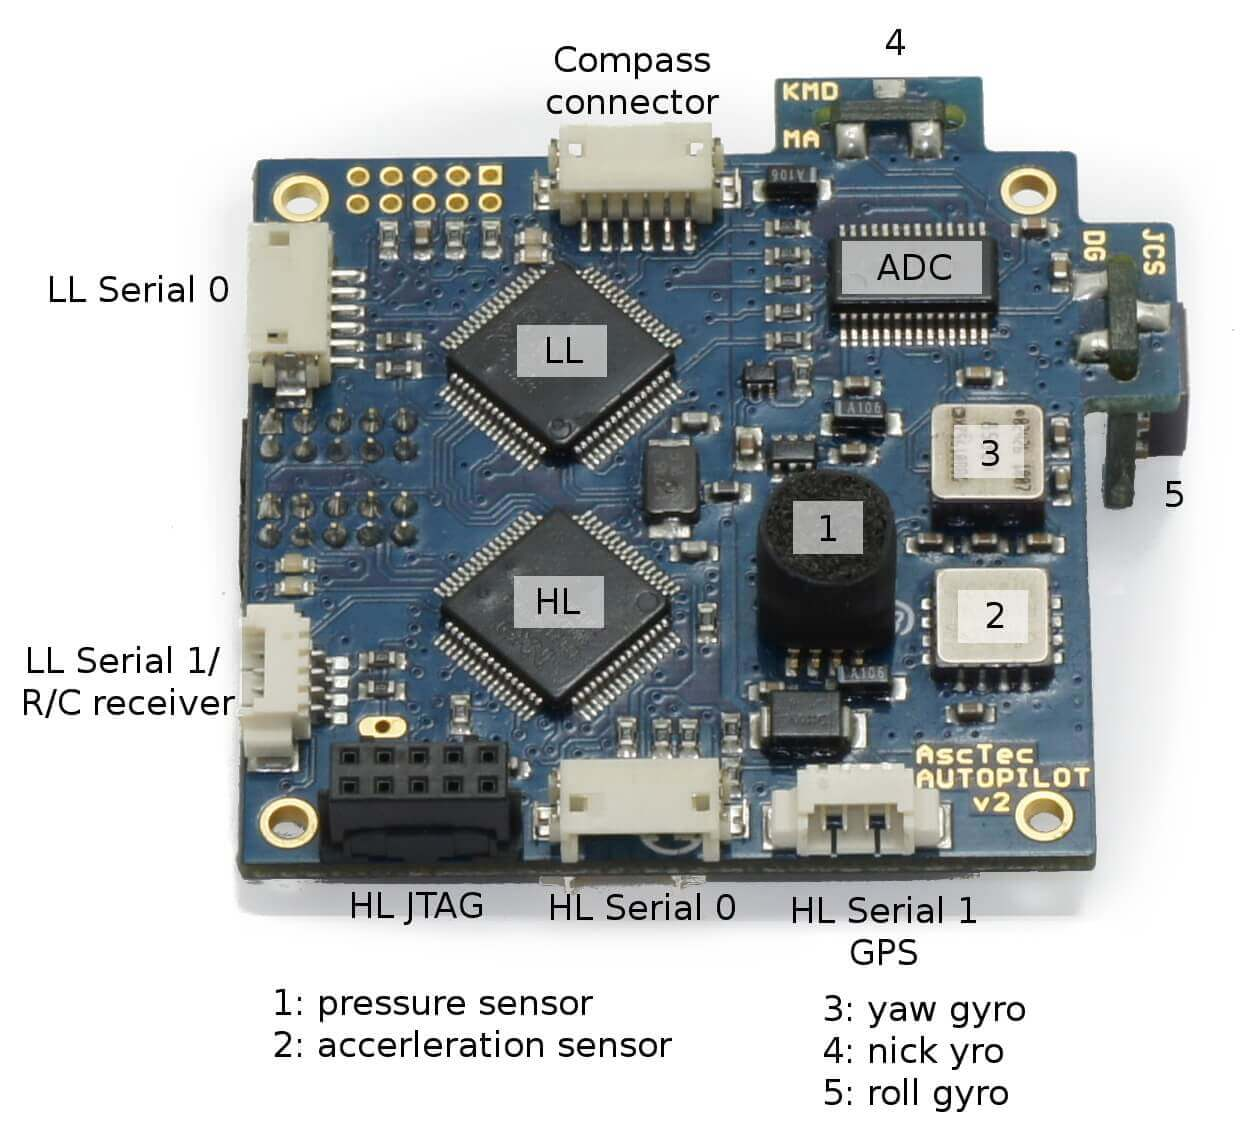}
	\caption{AscTec AutoPilot board pinout and connections \cite{asctec}}
	\label{fig:AutoPilotV2Desc}
\end{figure} 
 
Fig. \ref{fig:Powerboard} shows the pinout and connections of the AscTec Power Board.
\begin{figure}[!h]
	\centering
	\includegraphics[width=0.9\columnwidth]{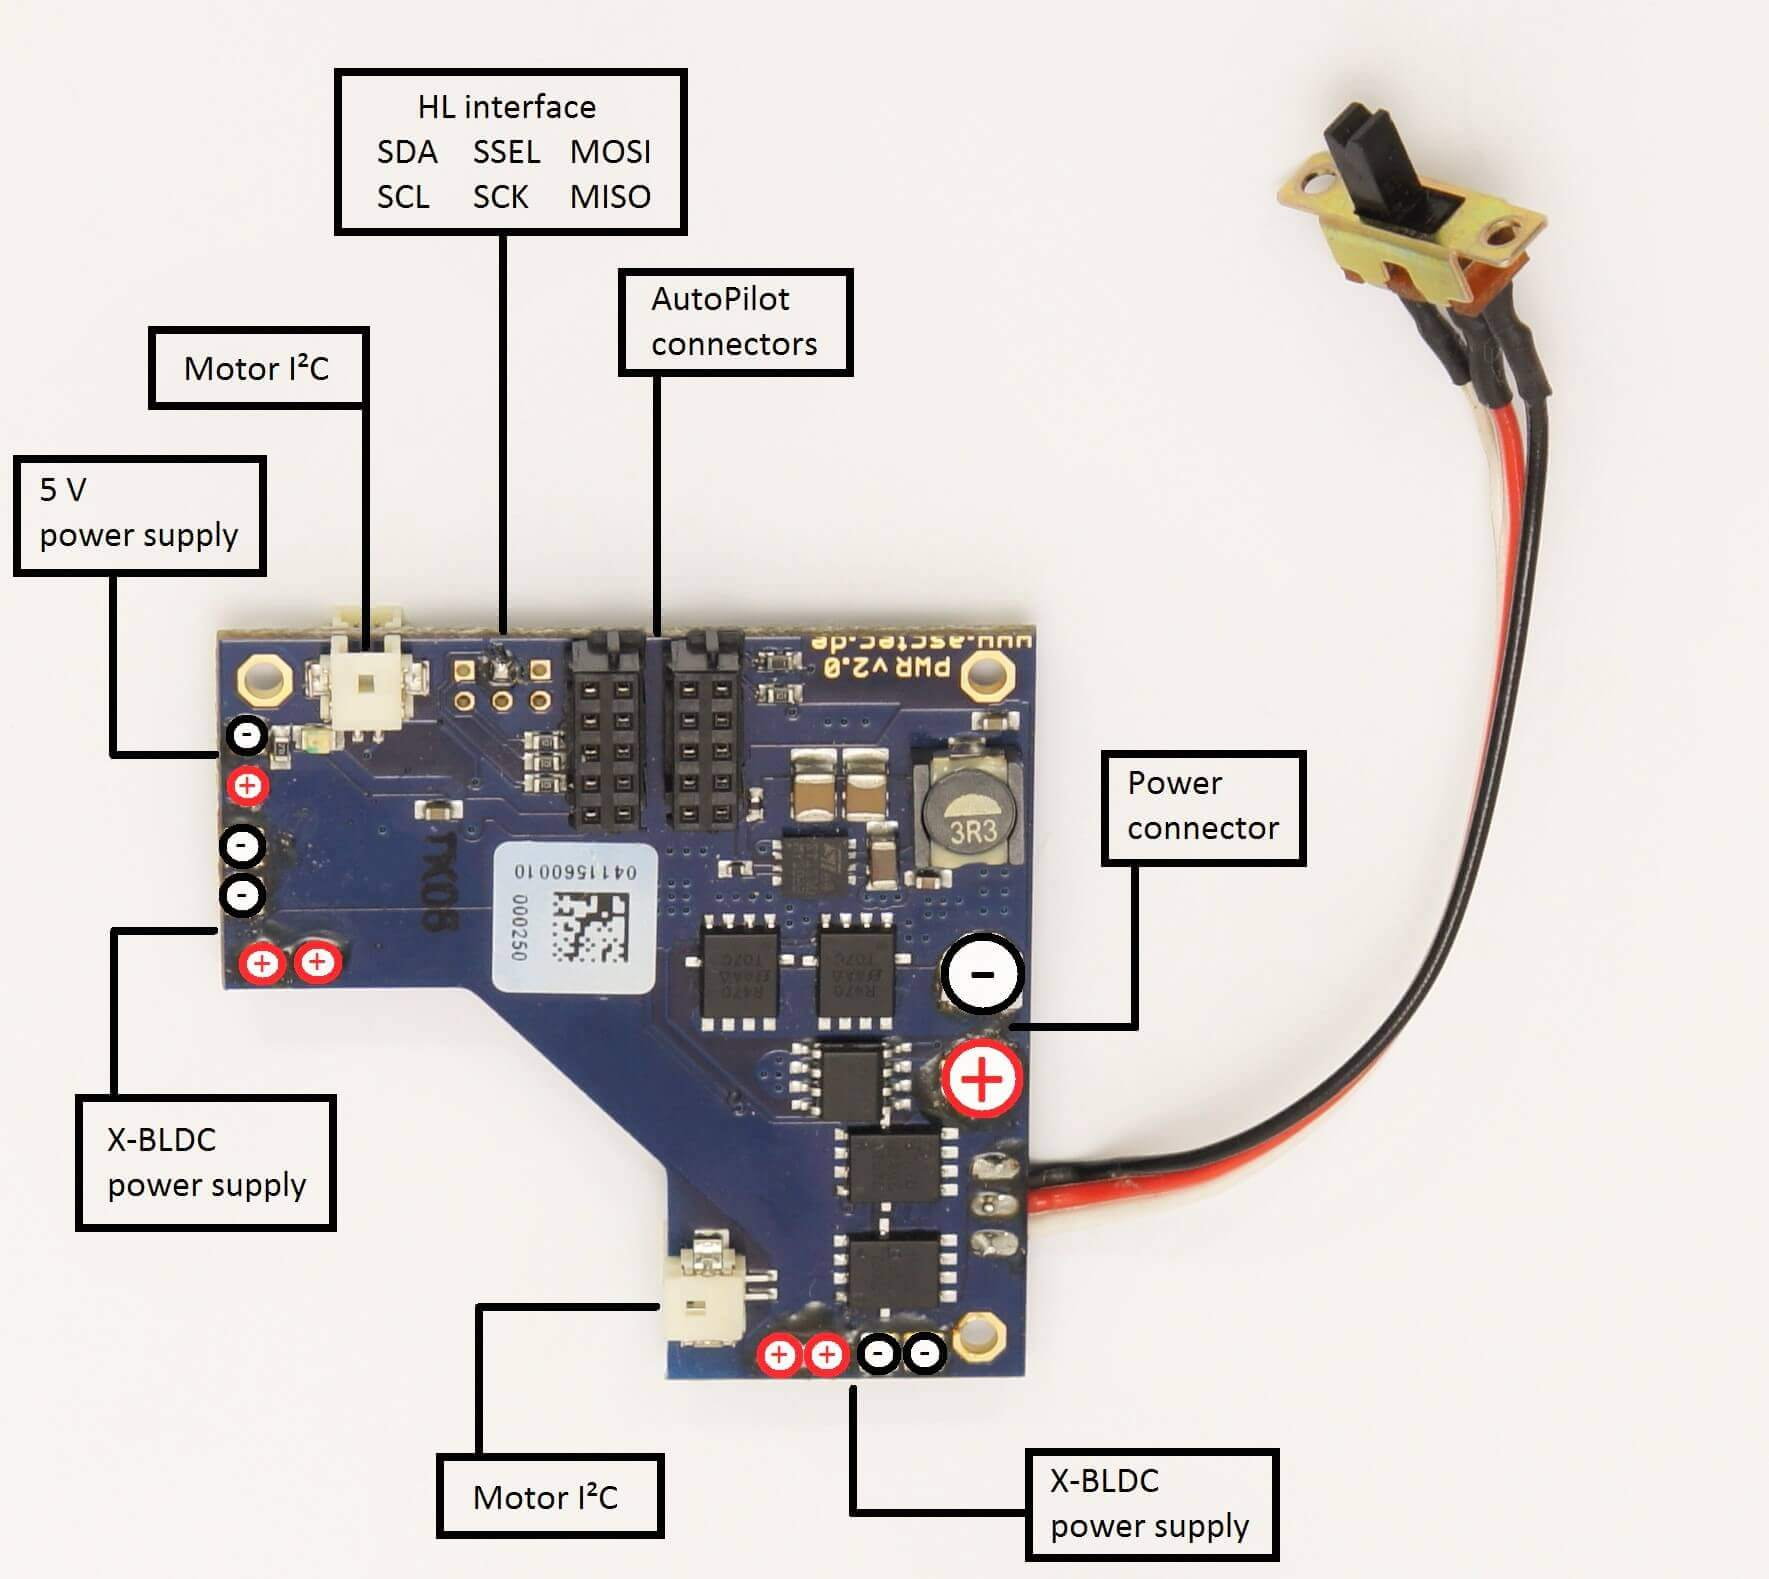}
	\caption{AscTec Power Board pinout and connections \cite{asctec}}
	\label{fig:Powerboard}
\end{figure} 
  
The AscTec Atomboard is the perfect choice for an x86-technology computer packed into a minimum form factor. By communicating with the AscTec Autopilot, IMU data can be included into your algorithms and high level commands can be sent to the flight system. Table \ref{tab:Atomboard_spec} presents the technical data of this onboard computer.

\begin{table}[!h]
	\caption{AscTec Atomboard technical specifications \cite{asctec}}
	\label{tab:Atomboard_spec}
	\begin{center}
		\begin{tabu}{|X|X|}
			\hline
			CPU & Intel® Atom™ Processor Z530 \\
			\hline
			CPU L2 Cache & 512k \\
			\hline
			Number of cores &  1 \\
			\hline
			Clock Speed & 1.6GHz \\
			\hline
			RAM  & 1GB DDR2 \\
			\hline
			GPU & Intel® GMA500 \\
			\hline
			Hard disk & 8GB SD Card \\ 
			\hline
			Display connector & LVDS \\
			\hline
			USB2.0 & 7x mini-USB A/B \\
			\hline
			UART & 2x\\
			\hline
		\end{tabu}
	\end{center}
\end{table} 
 
Fig. \ref{fig:atomboard-top} shows the top view of pinout and connections of the AscTec Atomboard (onboard computer).
\begin{figure}[!h]
	\centering
	\includegraphics[width=0.9\columnwidth]{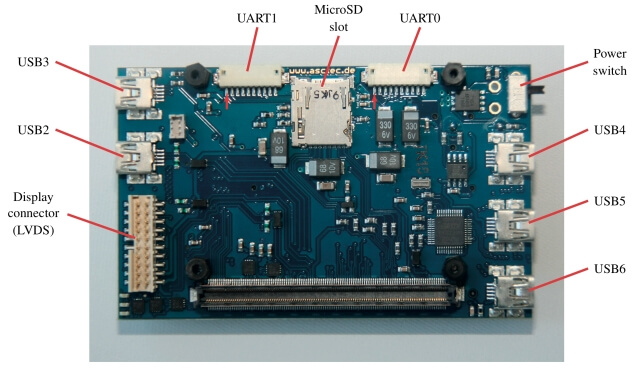}
	\caption{Top view of the onboard computer pinout and connections \cite{asctec}}
	\label{fig:atomboard-top}
\end{figure}   
 
Fig. \ref{fig:atomboard-bottom} shows the bottom view of pinout and connections of the AscTec Atomboard (onboard computer).
\begin{figure}[!h]
	\centering
	\includegraphics[width=0.9\columnwidth]{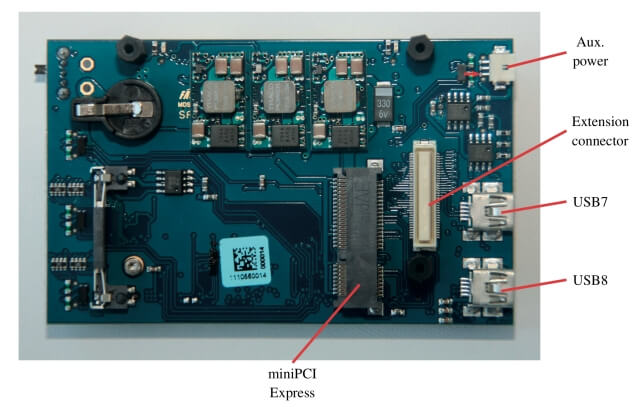}
	\caption{Bottom view of the onboard computer pinout and connections \cite{asctec}}
	\label{fig:atomboard-bottom}
\end{figure}
