# Supplementary material for: Controller Design and Implementation of a New Quadrotor Manipulation System
Source: arXiv:1904.08498 source file (2025-09-04)
Supplement: Supplementary file 6 [file Appendix_ros.tex]

\chapter{Robot Operating System (ROS)} \label{app:experimentalsystem-ros}

% change according to folder and file names
\ifpdf
    \graphicspath{{10_Appendices/figures/PNG/}{10_Appendices/figures/PDF/}{10_Appendices/figures/}}
\else
    \graphicspath{{10_Appendices/figures/EPS/}{10_Appendices/figures/}}
\fi

% ----------------------- contents from here ------------------------
\section{ROS}
ROS is an open-source, meta-operating system for your robot. It provides the
services you would expect from an operating system, including hardware abstraction, low-level device control, implementation of commonly-used functionality, message-passing between processes, and package management. It also provides tools and libraries for obtaining, building, writing, and running code across multiple computers.

\textbf{Why do we use ROS?}

There are specific issues in the development of software for robots that ROS can help to resolve, which are:
\begin{itemize}
	\item Distributed computation: Many modern robot systems rely on software that spans many different processes and runs across several different computers. For example: Some robots carry multiple computers, each of which controls a subset of the robot’s sensors or actuators. Even within a single computer, it’s often a good idea to divide the robot’s software into small, stand-alone parts that cooperate to achieve the overall goal. This approach is sometimes called "complexity via composition ".
	
	\item Software reuse: The rapid progress of robotics research has resulted in a growing collection of good algorithms for common tasks such as navigation, motion planning, mapping, and many others. Of course, the existence of these algorithms is only truly useful if there is a way to apply them in new contexts, without the need to reimplement each algorithm for	each new system. As a result, developers that use ROS can expect—after, of course, climbing ROS’s initial learning curve—to focus more time on experimenting with new ideas, and less time reinventing wheels.
	
	\item Rapid testing: One of the reasons that software development for robots is often more challenging than other kinds of development is that testing can be time consuming and error-prone. Physical robots may not always be available to work with, and when they are, the process is sometimes slow and finicky. Working with ROS provides two effective workarounds to this problem.
	\begin{itemize}
		\item  Well-designed ROS systems separate the low-level direct control of the hardware and high-level processing and decision making into separate programs. Because of this separation, we can temporarily replace those low-level programs (and their corresponding hardware) with a simulator, to test the behavior of the high-level part of
		the system.	
		\item ROS also provides a simple way to record and play back sensor data and other kinds
		of messages.
	\end{itemize}
	Therefore, because the real robot, the simulator, and the bag playback mechanism can all provide identical (or at least very similar) interfaces, your software does not need to be modified to operate in these distinct scenarios, and indeed need not even “know” whether it is talking to a real robot or to something else.
\end{itemize}

All ROS software is organized into packages. A ROS package is a coherent collection of files, generally including both executables (nodes) and supporting files, that serves a specific purpose. A robot control system comprises many nodes. For example, one node controls a laser range-finder, one Node controls the robot's wheel motors, one node performs localization. 

The primary mechanism that ROS nodes use to communicate is to send messages.
Messages in ROS are organized into named topics. The idea is that a node that wants to share information will publish messages on the appropriate topic; a node that wants to receive information will subscribe to the topic that it’s interested in. The ROS master takes care of ensuring that publishers and subscribers can find each other; the messages themselves are sent directly from publisher to subscriber.

\section{C++ Node for Extracting the Euler Angles from the Quaternion}
The ROS AscTec driver gives the quadrotor orientation in the form of quaternion. However, I need the roll and pitch angles to compensate the measured height from the sonar. Thus, I developed a ROS node to convert the quaternion to Euler angles.
\lstset {language=C++} 
\begin{lstlisting}
/****************************************************************************

Conversion from a quaternion to roll, pitch and yaw.

Nodes:
subscribed /rotation_quaternion (message of type geometry_msgs::Quaternion)
published /rpy_angles (message oftype geometry_msgs::Vector3.h)

****************************************************************************/

#include "ros/ros.h"
#include "geometry_msgs/Vector3.h"
#include "geometry_msgs/Quaternion.h"
#include "tf/transform_datatypes.h"
#include "LinearMath/btMatrix3x3.h"
#include <sensor_msgs/Imu.h>

// Here I use global publisher and subscriber, since I want to access the
// publisher in the function MsgCallback:
ros::Publisher rpy_publisher;
ros::Subscriber quat_subscriber;

// Function for conversion of quaternion to roll pitch and yaw. The angles
// are published here too.
void MsgCallback(const sensor_msgs::ImuPtr& msg)
{
	// the incoming geometry_msgs::Quaternion is transformed to a tf::Quaterion
	tf::Quaternion quat;
	tf::quaternionMsgToTF(msg->orientation, quat);
	
	// the tf::Quaternion has a method to acess roll pitch and yaw
	double roll, pitch, yaw;
	tf::Matrix3x3(quat).getRPY(roll, pitch, yaw);
	
	// the found angles are written in a geometry_msgs::Vector3
	geometry_msgs::Vector3 rpy;
	rpy.x = roll;
	rpy.y = pitch;
	rpy.z = yaw;
	
	// this Vector is then published:
	rpy_publisher.publish(rpy);
	ROS_INFO("published rpy angles: roll=%f pitch=%f yaw=%f", rpy.x, rpy.y, rpy.z);
}

int main(int argc, char **argv)
{
	ros::init(argc, argv, "talker");
	ros::NodeHandle n;
	rpy_publisher = n.advertise<geometry_msgs::Vector3>("rpy_angles", 1000);
	quat_subscriber = n.subscribe("rotation_quaternion", 1000, MsgCallback);
	
	// check for incoming quaternions untill ctrl+c is pressed
	ROS_INFO("waiting for quaternion");
	ros::spin();
	return 0;
}

\end{lstlisting}   

\section{ROS-based Arduino Code}

In the Arduino board, I write a program based on the rosserial library which enables me to communicate with ROS. Firstly, this C++ code reads the command from the WPS2 receiver, then process this command and then it to the SSC32 board via serial communications. Thirdly, it acquires and processes data from the sonar. Finally, it sends the height to the ROS.
  
\begin{lstlisting}
#include <DistanceSRF04.h>
#include <Wire.h>
#include <ros.h>
#include <geometry_msgs/Vector3.h>
#include <ros/time.h>
#include <std_msgs/Float32.h>
//=============== manp ===================
#include <PS2X_lib.h> 
#define PS2_DAT        5  //14    
#define PS2_CMD        4  //15
#define PS2_SEL        3  //16
#define PS2_CLK        2  //17
//#define pressures   true
#define pressures   false
//#define rumble      true
#define rumble      false
PS2X ps2x;
int error = 0;
byte type = 0;
byte vibrate = 0;
int angle0 = 90;
int angle1 = 90;
int grasp = 90;
int angle0_pwm;
int angle1_pwm;
int grasp_pwm;
int joint0_ch=0;
int joint1_ch=4;
int grasp_ch=8;
int anglestep =1;
int time = 1;
//=======================================

std_msgs::Float32 sonar_msg;
ros::Publisher pub_sonar("sonar", &sonar_msg);
ros::NodeHandle nh;

DistanceSRF04 Dist;
void setup()
{
Dist.begin(8,9);
nh.initNode();
nh.advertise(pub_sonar);

// ================= Manp ================
Serial1.begin(115200);
delay(500); 
error = ps2x.config_gamepad(PS2_CLK, PS2_CMD, PS2_SEL, PS2_DAT,
 pressures, rumble);
type = ps2x.readType(); 
// ======================================
}

long publisher_timer;

void loop()
{
  if (millis() > publisher_timer) {
sonar_msg.data = Dist.getDistancemeter();

  pub_sonar.publish(&sonar_msg);
  publisher_timer = millis() + 100; //publish once a second
}
manp();
nh.spinOnce();
}

// ======================== Manp Functions =================
void manp()
{
if(error == 1) //skip loop if no controller found
return; 

if(type == 2){ //Guitar Hero Controller
ps2x.read_gamepad();          //read controller 
}
else { //DualShock Controller
ps2x.read_gamepad(false, vibrate); //read controller and set large 
motor to spin at 'vibrate' speed     

if(ps2x.Button(PSB_PAD_UP))      //will be TRUE as long as button is
 pressed
angle0 +=anglestep;
//=============================================================================================    
if(ps2x.Button(PSB_PAD_DOWN))
angle0 -=anglestep;
//=============================================================================================    
if(ps2x.Button(PSB_PAD_RIGHT))
angle1 +=anglestep;

//=============================================================================================    
if(ps2x.Button(PSB_PAD_LEFT)){
angle1 -=anglestep;
Serial1.print("pressures = ");
}
if(angle0<0) angle0=0;
if(angle0>180) angle0=180;
if(angle1<0) angle1=0;
if(angle1>180) angle1=180;

angle0_pwm= map(angle0, 0, 180, 500, 2500);
move(joint0_ch,angle0_pwm, time);
angle1_pwm= map(angle1, 0, 180, 500, 2500);
move(joint1_ch,angle1_pwm, time);

vibrate = ps2x.Analog(PSAB_CROSS);  //this will set the large motor
 vibrate speed based on how hard you press the blue (X) button

if(ps2x.Button(PSB_L1) || ps2x.Button(PSB_R1)) { //print stick values if
 either is TRUE
if(ps2x.Button(PSB_L1)) { //print stick values if either is TRUE

grasp-=anglestep;
}
if(ps2x.Button(PSB_R1)) { //print stick values if either is TRUE

grasp+=anglestep;
} 
} 
if(grasp<0) grasp=0;
if(grasp>180) grasp=180; 
grasp_pwm= map(grasp, 0, 180, 500, 2500);
move(grasp_ch,grasp_pwm, time);    
}
delay(50); 
}

void move(int servo, int position, int time) {
Serial1.print("#");
Serial1.print(servo);
Serial1.print(" P");
Serial1.print(position);
Serial1.print(" T");
Serial1.println(time);
delay(time);
}
\end{lstlisting} 
\section{Altitude Compensation Node}
This node receives the height from the Arduino and then it compensates the altitude based on the measured roll and pitch angles.
\begin{lstlisting} 
#include "ros/ros.h"
#include <ros/time.h>
#include "geometry_msgs/Vector3.h"
#include "mav_msgs/Height.h"
#include "std_msgs/Float32.h"
//#include "var.h"

ros::Publisher alt_pub;
ros::Subscriber sonar_sub;
ros::Subscriber rpy_sub;
float sonar_alt, ph, th;
char frameid[] = "";

void MsgCallback(const std_msgs::Float32& sonar_msg)
{
sonar_alt= sonar_msg.data;
return;
}

void MsgCallbackrpy(const geometry_msgs::Vector3& rpy_msg)
{
ph=rpy_msg.x;
th=rpy_msg.y;
return;
}
int main(int argc, char **argv)
{
ros::init(argc, argv, "altitude");
ros::NodeHandle n;
sonar_sub = n.subscribe("sonar", 5, MsgCallback);
rpy_sub = n.subscribe("rpy_angles", 5, MsgCallbackrpy);
alt_pub = n.advertise<mav_msgs::Height>("alt", 5);
ros::Rate loop_rate(10);
while (ros::ok())
{
mav_msgs::Height alt_msg;
alt_msg.height =  sonar_alt*cos(ph)*cos(th);
alt_msg.header.stamp = ros::Time::now();
alt_msg.header.frame_id =  frameid;
alt_msg.height_variance = 0;  
alt_msg.climb= 0.0;
alt_msg.climb_variance= 0;
alt_pub.publish(alt_msg);
ros::spinOnce();
loop_rate.sleep();
}
ros::spin();
return 0;
}

\end{lstlisting} 
\section{Joystick teleoperation Node}
This node reads the joystick buttons and converts them to position and velocity commands.
\begin{lstlisting} 
#include <ros/ros.h>
#include <sensor_msgs/Joy.h>
#include <std_msgs/Bool.h>
#include <std_msgs/Float32.h>
#include <stdlib.h>
ros::Subscriber joy_sub ;
ros::Publisher x_pub;
ros::Publisher y_pub;
ros::Publisher z_pub;
ros::Publisher ep_pub;
ros::Publisher reset_pub;
ros::Publisher zvel_pub;
//last_joy_event_ = ros::Time::now();

float x_step_size=0.01; 
float x_old=0;
float x_delta=0;
float y_step_size=0.01; 
float y_old=0;
float y_delta=0;
float z_step_size=0.01; 
float z_old=0;
float z_delta=0;
float z_min=0;
float ep_step_size=0.01; 
float ep_old=0;
float ep_delta=0;
float zvel_step_size=0.01; 
float zvel_old=0;
float zvel_delta=0;
float zvel_min=0;
bool sw=0;
bool b0,b1,b2,b3,b5,b7,b8,b10,b11,b4,b6,b9;
// **** 
void joyCallback(const sensor_msgs::JoyPtr& joy_msg)
{ // start of callback
b0=joy_msg->buttons[0];
b1=joy_msg->buttons[1];
b2=joy_msg->buttons[2];
b3=joy_msg->buttons[3];
b5=joy_msg->buttons[5];
b7=joy_msg->buttons[7];
b8=joy_msg->buttons[8];
b10=joy_msg->buttons[10];
b11=joy_msg->buttons[11];
b4=joy_msg->buttons[4];
b6=joy_msg->buttons[6];
b9=joy_msg->buttons[9];
//=============================
std_msgs::Float32 x_msg;
std_msgs::Float32 y_msg;
std_msgs::Float32 z_msg;
std_msgs::Float32 ep_msg;
std_msgs::Bool reset_msg;
std_msgs::Float32 zvel_msg;
// ================== x-axis ==============================
if (b0  ==1 || b2 == 1)
{
if (b0 == 1)
{
x_delta= x_step_size ;
}
else if (b2 == 1)
{
x_delta= -x_step_size ; 
}

x_msg.data =    x_old + x_delta;
x_old=x_msg.data;
}
else {x_msg.data = x_old;}
// =======================================================

// ================== y-axis ==============================
if (b3 ==1 || b1 == 1)
{
if (b3 == 1)
{
y_delta= y_step_size ;
}
else if (b1 == 1)
{
y_delta= -y_step_size ; 
}

y_msg.data =    y_old + y_delta;
y_old=y_msg.data;
}
else {y_msg.data = y_old;}
// =======================================================

// ================== z-axis ==============================
if (b5 ==1 || b7 == 1)
{
if (b5 == 1)
{
z_delta= z_step_size ;
}
else if (b7 == 1)
{
z_delta= -z_step_size ; 
}

z_msg.data =  z_old + z_delta;
z_msg.data = std::max(z_msg.data, z_min);
z_old=z_msg.data;
}
else {z_msg.data = z_old;}

// =======================================================

// ================== ep-axis ==============================
if (b11 ==1 || b10 == 1)
{
if (b11 == 1)
{
ep_delta= ep_step_size ;
}
else if (b10 == 1)
{
ep_delta= -ep_step_size ; 
}

ep_msg.data =  ep_old + ep_delta;

ep_old=ep_msg.data;
}
else {ep_msg.data = ep_old;}

// =======================================================

// ================== reset ==============================

if (b9 ==1 || sw==1 && b8==0) {reset_msg.data=1; sw=1;}
else {reset_msg.data=0; sw=0;}

// =======================================================
// ================== zvel-axis ==============================
if (b4  ==1 || b6 == 1)
{
if (b4 == 1)
{
zvel_delta= zvel_step_size ;
}
else if (b6 == 1)
{
zvel_delta= -zvel_step_size ; 
}

zvel_msg.data =    zvel_old + zvel_delta;
zvel_old=zvel_msg.data;
}
else {zvel_msg.data = zvel_old;}
// =======================================================

x_pub.publish(x_msg);
y_pub.publish(y_msg);
z_pub.publish(z_msg);
ep_pub.publish(ep_msg);
reset_pub.publish(reset_msg);
zvel_pub.publish(zvel_msg);
//==================================
return;
} // end of call back

int main(int argc, char ** argv)
{  
ros::init(argc, argv, "quad_joy_teleop");
ros::NodeHandle nh;
x_pub = nh.advertise<std_msgs::Float32>("x_des", 5);
y_pub = nh.advertise<std_msgs::Float32>("y_des", 5);
z_pub = nh.advertise<std_msgs::Float32>("z_des", 5);
ep_pub = nh.advertise<std_msgs::Float32>("ep_des", 5);
reset_pub = nh.advertise<std_msgs::Bool>("reset_des", 5);
zvel_pub = nh.advertise<std_msgs::Float32>("zvel_des", 5);
joy_sub= nh.subscribe("joy", 5, joyCallback);
ros::spin();
return 0;
}
\end{lstlisting}
