# Supplementary material for: Controller Design and Implementation of a New Quadrotor Manipulation System
Source: arXiv:1904.08498 source file (2025-09-04)
Supplement: Supplementary file 7 [file Appendix_sonar.tex]

\chapter{Ultrasonic Ranger} \label{app:experimentalsystem-sonar}

% change according to folder and file names
\ifpdf
    \graphicspath{{10_Appendices/figures/PNG/}{10_Appendices/figures/PDF/}{10_Appendices/figures/}}
\else
    \graphicspath{{10_Appendices/figures/EPS/}{10_Appendices/figures/}}
\fi

% ----------------------- contents from here ------------------------

The Devantech SRF04 ultrasonic range finder (see Fig. \ref{fig:devantech-srf04-ultrasonic-range-finder}) provides precise, non-contact distance measurements from about 3 cm to 3 m. The SRF04 works by transmitting an ultrasonic (well above human hearing range) pulse and measuring the time it takes to "hear" the pulse echo. Output from the SRF04 is in the form of a variable-width pulse that corresponds to the distance to the target.
\begin{figure}[!h]
	\centering
	\includegraphics[width=0.5\columnwidth]{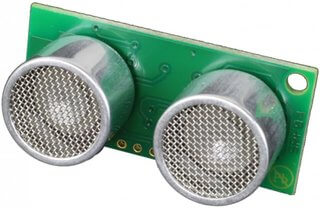}
	\caption{Devantech SRF04 Ultrasonic Range Finder \cite{sonar_ref}}
	\label{fig:devantech-srf04-ultrasonic-range-finder}
\end{figure}
Technical specifications of this device is given in Table \ref{tab:sonar_spec}.
\begin{table}[!h]
	\caption{Ultrasonic, SRF04, technical specifications \cite{sonar_ref}}
	\label{tab:sonar_spec}
	\begin{center}
		\begin{tabu}{|X|X|}
			\hline
		Sensor type & Reflective Ultrasonic \\
		\hline
		Sender & N1076, Receiver N1081 \\
		\hline
		Voltage &  5v only required \\
		\hline
		Current & 30mA Typical, 50mA Max. \\
		\hline
		Frequency  & 40kHz \\
		\hline
		Range & 3cm - 3m \\
		\hline
		Sensitivity & Detect 3cm diameter \\
		\hline
		Input Trigger & 10uS Min. TTL (Transistor Transistor Logic) level pulse \\ 
		\hline
		Echo Pulse & Positive TTL level signal, width proportional to range \\
		\hline
		I/O required & two digital lines, 1 output, 1 input \\
		\hline
		Small Size & 43mm x 20mm x 17mm height\\
		\hline
		Weight & 11.33 gm \\ 
			\hline
		\end{tabu}
	\end{center}
\end{table}

Fig. \ref{fig:sonar_dim} illustrates schematic diagrams of the sonar with the relevant dimensions.
\begin{figure}[!h]
	\centering
	\includegraphics[width=0.6\columnwidth]{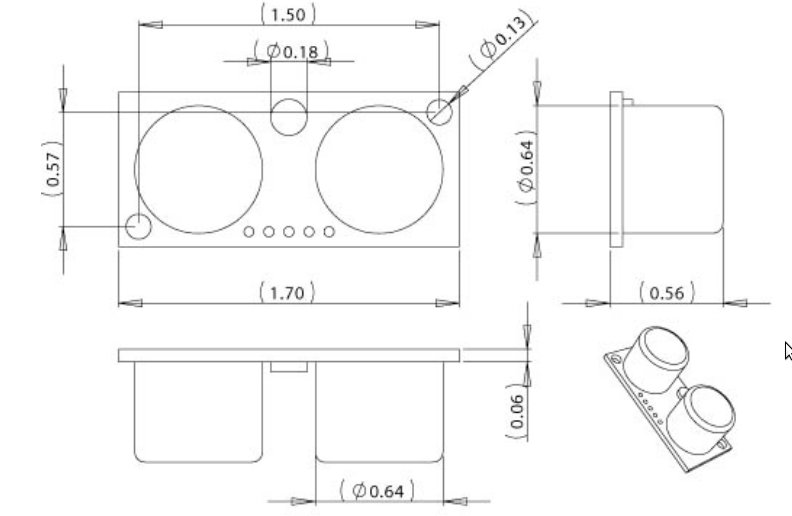}
	\caption{External dimension of the SRF04 \cite{sonar_ref}}
	\label{fig:sonar_dim}
\end{figure}

Fig. \ref{fig:sonar_conn} shows the terminal connections of the sonar.
\begin{figure}[!h]
	\centering
	\includegraphics[width=0.6\columnwidth]{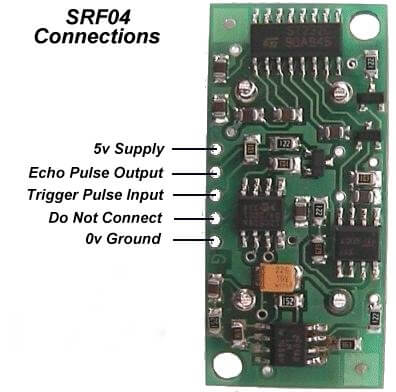}
	\caption{Terminal Connections of the SRF04 \cite{sonar_ref}}
	\label{fig:sonar_conn}
\end{figure}

The SRF04 beam pattern is given in Fig. \ref{fig:sonar_beam}. Its Timing diagram is shown in Fig. \ref{fig:sonar_time}. We only need to supply a short 10 $\mu s$ pulse to the trigger input to start the ranging. The SRF04 will send out an 8 cycle burst of ultrasound at 40khz and raise its echo line high. It then listens for an echo, and as soon as it detects one it lowers the echo line again. The echo line is therefore a pulse whose width is proportional to the distance to the object. By timing the pulse it is possible to calculate the range in inches/centimeters or anything else.  If the width of the pulse is measured in $\mu s$, then dividing by 58 will give you the distance in cm.

\begin{figure}[!h]
	\centering
	\includegraphics[width=0.8\columnwidth]{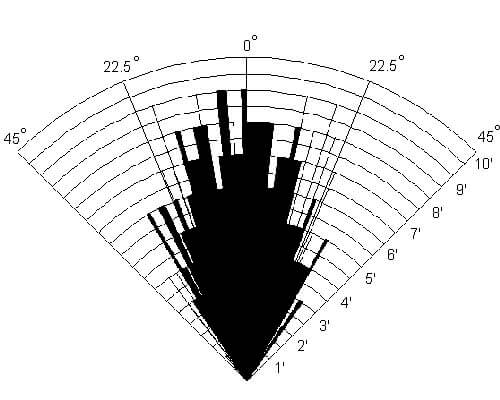}
	\caption{Beam Pattern of the SRF04 \cite{sonar_ref}}
	\label{fig:sonar_beam}
\end{figure}

\begin{figure}[!h]
	\centering
	\includegraphics[width=0.8\columnwidth]{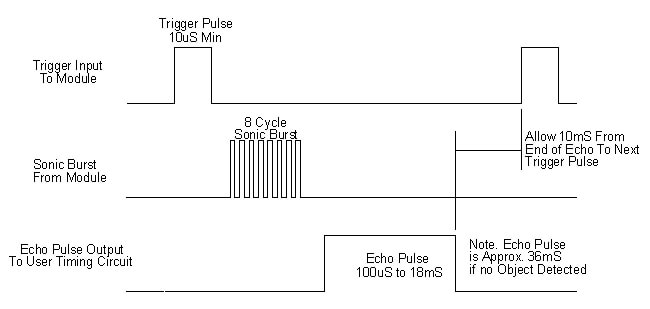}
	\caption{Timing diagram of the SRF04 \cite{sonar_ref}}
	\label{fig:sonar_time}
\end{figure}
