# Supplementary material for: Controller Design and Implementation of a New Quadrotor Manipulation System
Source: arXiv:1904.08498 source file (2025-09-04)
Supplement: Supplementary file 8 [file Appendix_tfsensor.tex]

\chapter{6-DOF Torque/Force Sensor} \label{app:experimentalsystem-tfsensor} 

% change according to folder and file names
\ifpdf
    \graphicspath{{10_Appendices/figures/PNG/}{10_Appendices/figures/PDF/}{10_Appendices/figures/}}
\else
    \graphicspath{{10_Appendices/figures/EPS/}{10_Appendices/figures/}}
\fi

% ----------------------- contents from here ------------------------
We use a torque force sensor of model, IFS-67M25A25-I40ANA, see Fig. \ref{fig:tfsens}. In this sensor, foil strain gages sense the loads imposed on the sensor. The strain gage signals are amplified and combined to become analog representations of the force loads on the three axes and the moments or torques about the three axes. 

\begin{figure}[!h]
	\centering
	\includegraphics[width=0.9\columnwidth]{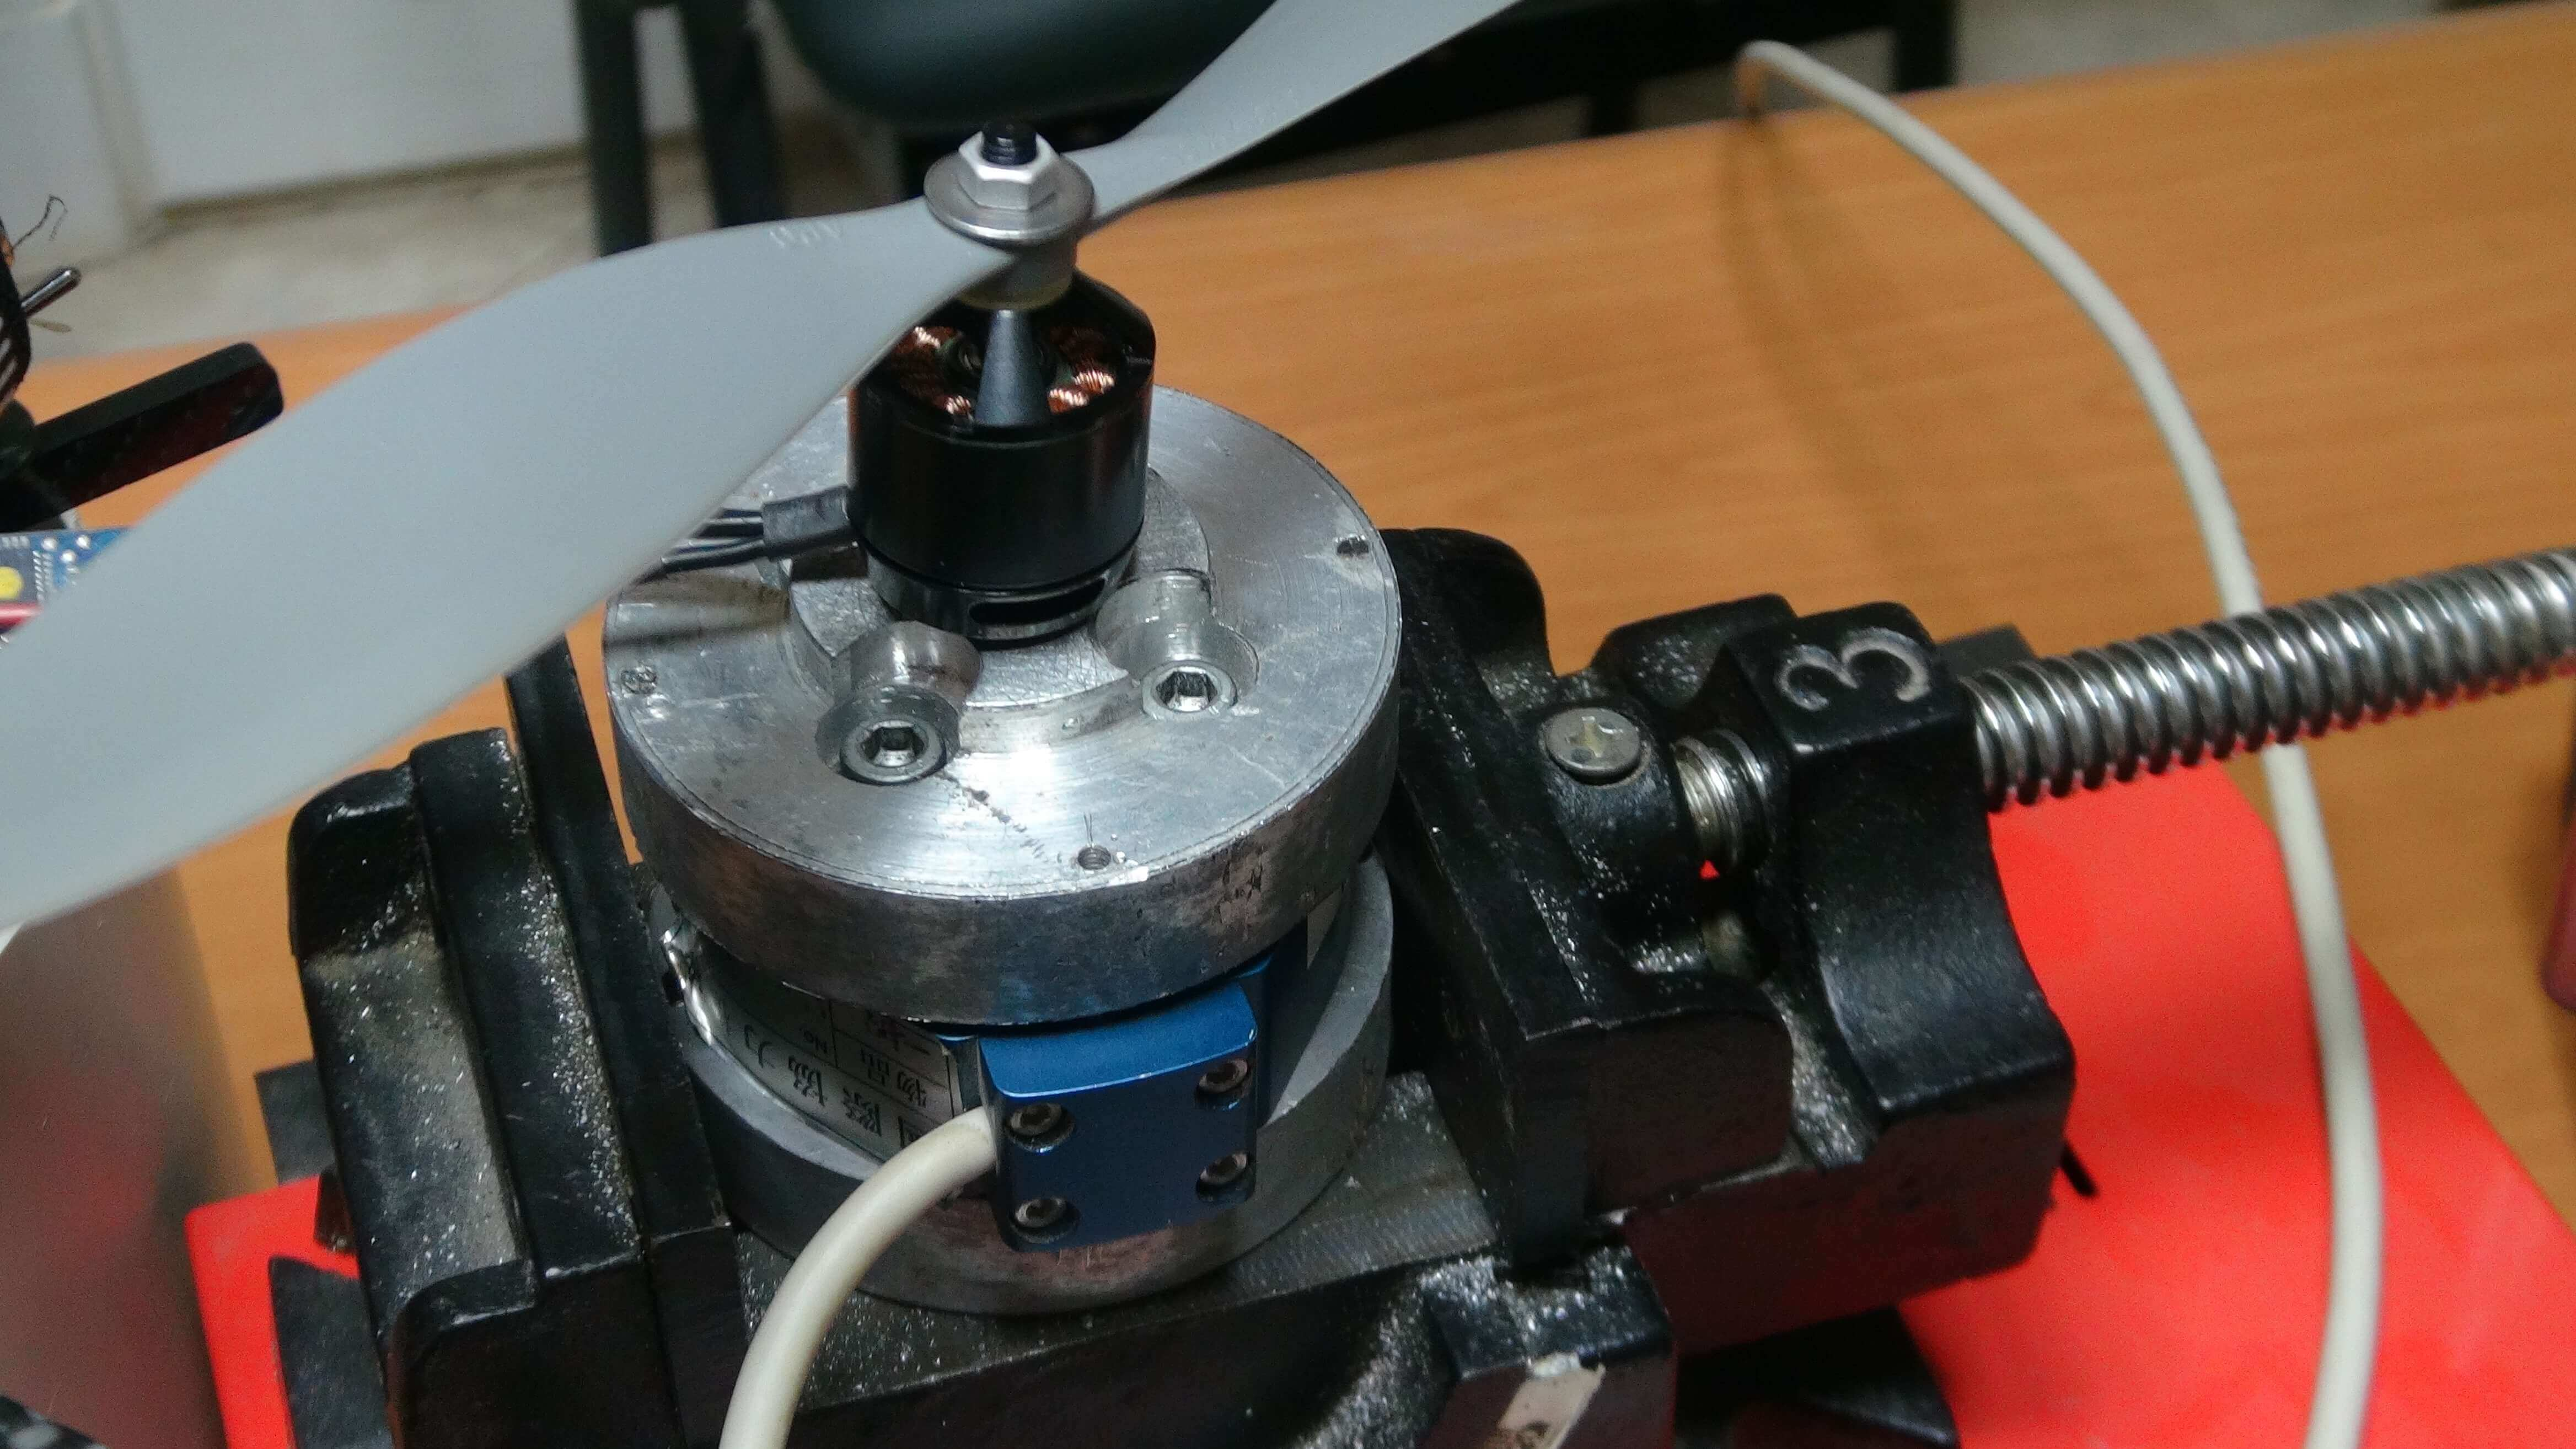}
	\caption{The Torque Force sensor with the interface mount to rotor to be identified}
	\label{fig:tfsens}
\end{figure}
Fig. \ref{fig:tfsens_orient} presents the sensor axis orientation from the rotor side.
\begin{figure}[!h]
	\centering
	\includegraphics[width=0.5\columnwidth]{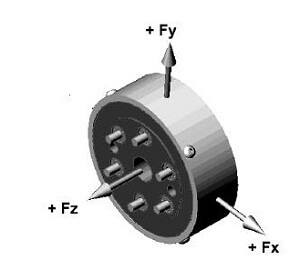}
	\caption{Torque/Force sensor axis orientation from the rotor side \cite{tfsens_ref}}
	\label{fig:tfsens_orient}
\end{figure}

It utilizes a DE-9P connector to produce the analogue output. The pin assignment is given in Table \ref{tab:tfsnes_pin}. 

\begin{table}[!h]
	\caption{Pin Connections of the 6-DOF torque/force sensor \cite{tfsens_ref}}
	\label{tab:tfsnes_pin}
	\begin{center}
		\begin{tabu}{|X|X|}
			\hline
	PIN & SIGNAL\\
		\hline
	1 & $F_x$ \\
	\hline
	2 & $F_y$\\
	\hline
	3 & $F_z$\\
	\hline
	4 & $M_x$\\
	\hline
	5 & $M_y$\\
	\hline
	6 & $M_z$\\
	\hline
	7 & + power, Sensor excitation: $\pm$5.0V\\
	\hline
	8 & - power\\
	\hline
	9 &	power and signal common \\		
			\hline
  \end{tabu}
\end{center}
\end{table}

Data from analog sensors must be processed using the Calibration Matrix provided with the sensor.

The six by six calibration matrix is multiplied by the six element
voltage (column) vector. The result is the calibrated force and moment data in the units of N and Nm. Multiply the calibration matrix and the sensor  voltage vector to determine the loads (N and Nm).

$$
\begin{bmatrix}
F_x\\
F_y\\
F_z\\
M_x\\
M_y\\
M_z\\
\end{bmatrix}
=
\begin{bmatrix}
49.487& -1.552& -0.671& -4.053& -1.636& -0.043\\
1.852& 49.666& -0.483& 1.450& -2.442& -1.495\\
-1.695& 2.721& 86.221& 1.107& -0.006& 0.081\\
 0.000& 0.121& 0.026& 2.904& 0.140& 0.032\\
 -0.135& 0.001& 0.018& -0.058& 0.024& 0.064\\ 
 -0.128& 0.012& 2.800& 0.033& -0.098& 3.042\\
\end{bmatrix}
\times
\begin{bmatrix}
F_x voltage\\
F_y voltage\\
F_z voltage\\
M_x voltage\\
M_y voltage\\
M_z voltage\\
\end{bmatrix}
$$
