# Supplementary material for: Controller Design and Implementation of a New Quadrotor Manipulation System
Source: arXiv:1904.08498 source file (2025-09-04)
Supplement: Supplementary file 9 [file Appendix.tex]

\begin{Appendices}
   	
\end{Appendices}
