# Supplementary material for: Controller Design and Implementation of a New Quadrotor Manipulation System
Source: arXiv:1904.08498 source file (2025-09-04)
Supplement: Supplementary file 10 [file Appendix_forkin.tex]

\chapter{Forward Kinematics} 
\label{app:forwardkinematics}

% change according to folder and file names
\ifpdf
    \graphicspath{{10_Appendices/figures/PNG/}{10_Appendices/figures/PDF/}{10_Appendices/figures/}}
\else
    \graphicspath{{10_Appendices/figures/EPS/}{10_Appendices/figures/}}
\fi

% ----------------------- contents from here ------------------------
\lstset {language=Matlab} 
\begin{lstlisting}
function Xe = For_Kin(zt,sb)
L0 = 30e-03;
L1 = 70e-03;
L2 = 85e-03; 
X = zt(1);
Y = zt(2);
Z = zt(3);
ep = zt(4);
th1 = zt(5);
th2 = zt(6);
ph = sb(2);
th = sb(1);
%% ================================= 
% A0_B = Transformation matrix from frame 0 to frame B
A0_B = [0 0 1 0; -1 0 0 0; 0 -1 0 -L0; 0 0 0 1]; 
A1_0 = [cos(th1) 0 sin(th1) L1*cos(th1); sin(th1) 0 -cos(th1) L1*sin(th1); 
0 1 0 0; 0 0 0 1]; 
A2_1 = [cos(th2) -sin(th2) 0 L2*cos(th2); sin(th2) cos(th2) 0 L2*sin(th2); 
0 0 1 0; 0 0 0 1];
AB_I = [cos(ep)*cos(th), cos(ep)*sin(ph)*sin(th)-cos(ph)*sin(ep),
 sin(ep)*sin(ph)+cos(ep)*cos(ph)*sin(th),X;
cos(th)*sin(ep), cos(ep)*cos(ph)+sin(ep)*sin(ph)*sin(th),
 cos(ph)*sin(ep)*sin(th)-cos(ep)*sin(ph),Y;
-sin(th), cos(th)*sin(ph), cos(ph)*cos(th),Z;
0,0, 0, 1]; 
T2_I = AB_I* A0_B * A1_0 * A2_1;
% T2_I = eval(T2_I);
xe = T2_I(1,4);
ye = T2_I(2,4);
ze = T2_I(3,4);
%% Computing Euler angles from a rotation matrix
R31 = T2_I(3,1);
R32 = T2_I(3,2);
R33 = T2_I(3,3);
R21 = T2_I(2,1);
R11 = T2_I(1,1);
R12 = T2_I(1,2);
R13 = T2_I(1,3);
if (R31~=+1 \&\& R31~=-1)
the = -asin(R31); 
%or
% the = pi - (-asin(R31))
phe = atan2(R32/cos(the),R33/cos(the)); 
epe = atan2(R21/cos(the),R11/cos(the)); 
else
epe =0; %anything; can set to 0
if (R31 == -1)
the = pi/2;
phe = epe + atan2(R12,R13);
else
the = -pi/2;
phe = -epe + atan2(-R12, -R13);
end
end
Xe = [xe;ye;ze;epe;the;phe];
end
\end{lstlisting}
