# Supplementary material for: Controller Design and Implementation of a New Quadrotor Manipulation System
Source: arXiv:1904.08498 source file (2025-09-04)
Supplement: Supplementary file 11 [file Appendix_power.tex]

\chapter{System Internal Connections} \label{app:experimentalsystem-power}

% change according to folder and file names
\ifpdf
    \graphicspath{{10_Appendices/figures/PNG/}{10_Appendices/figures/PDF/}{10_Appendices/figures/}}
\else
    \graphicspath{{10_Appendices/figures/EPS/}{10_Appendices/figures/}}
\fi

% ----------------------- contents from here ------------------------

Internal connections (i.e., power and data connections) of the proposed robot are given in Fig. \ref{fig:power_conn}
\begin{figure}[!h]
	\centering
	\includegraphics[width=1\columnwidth]{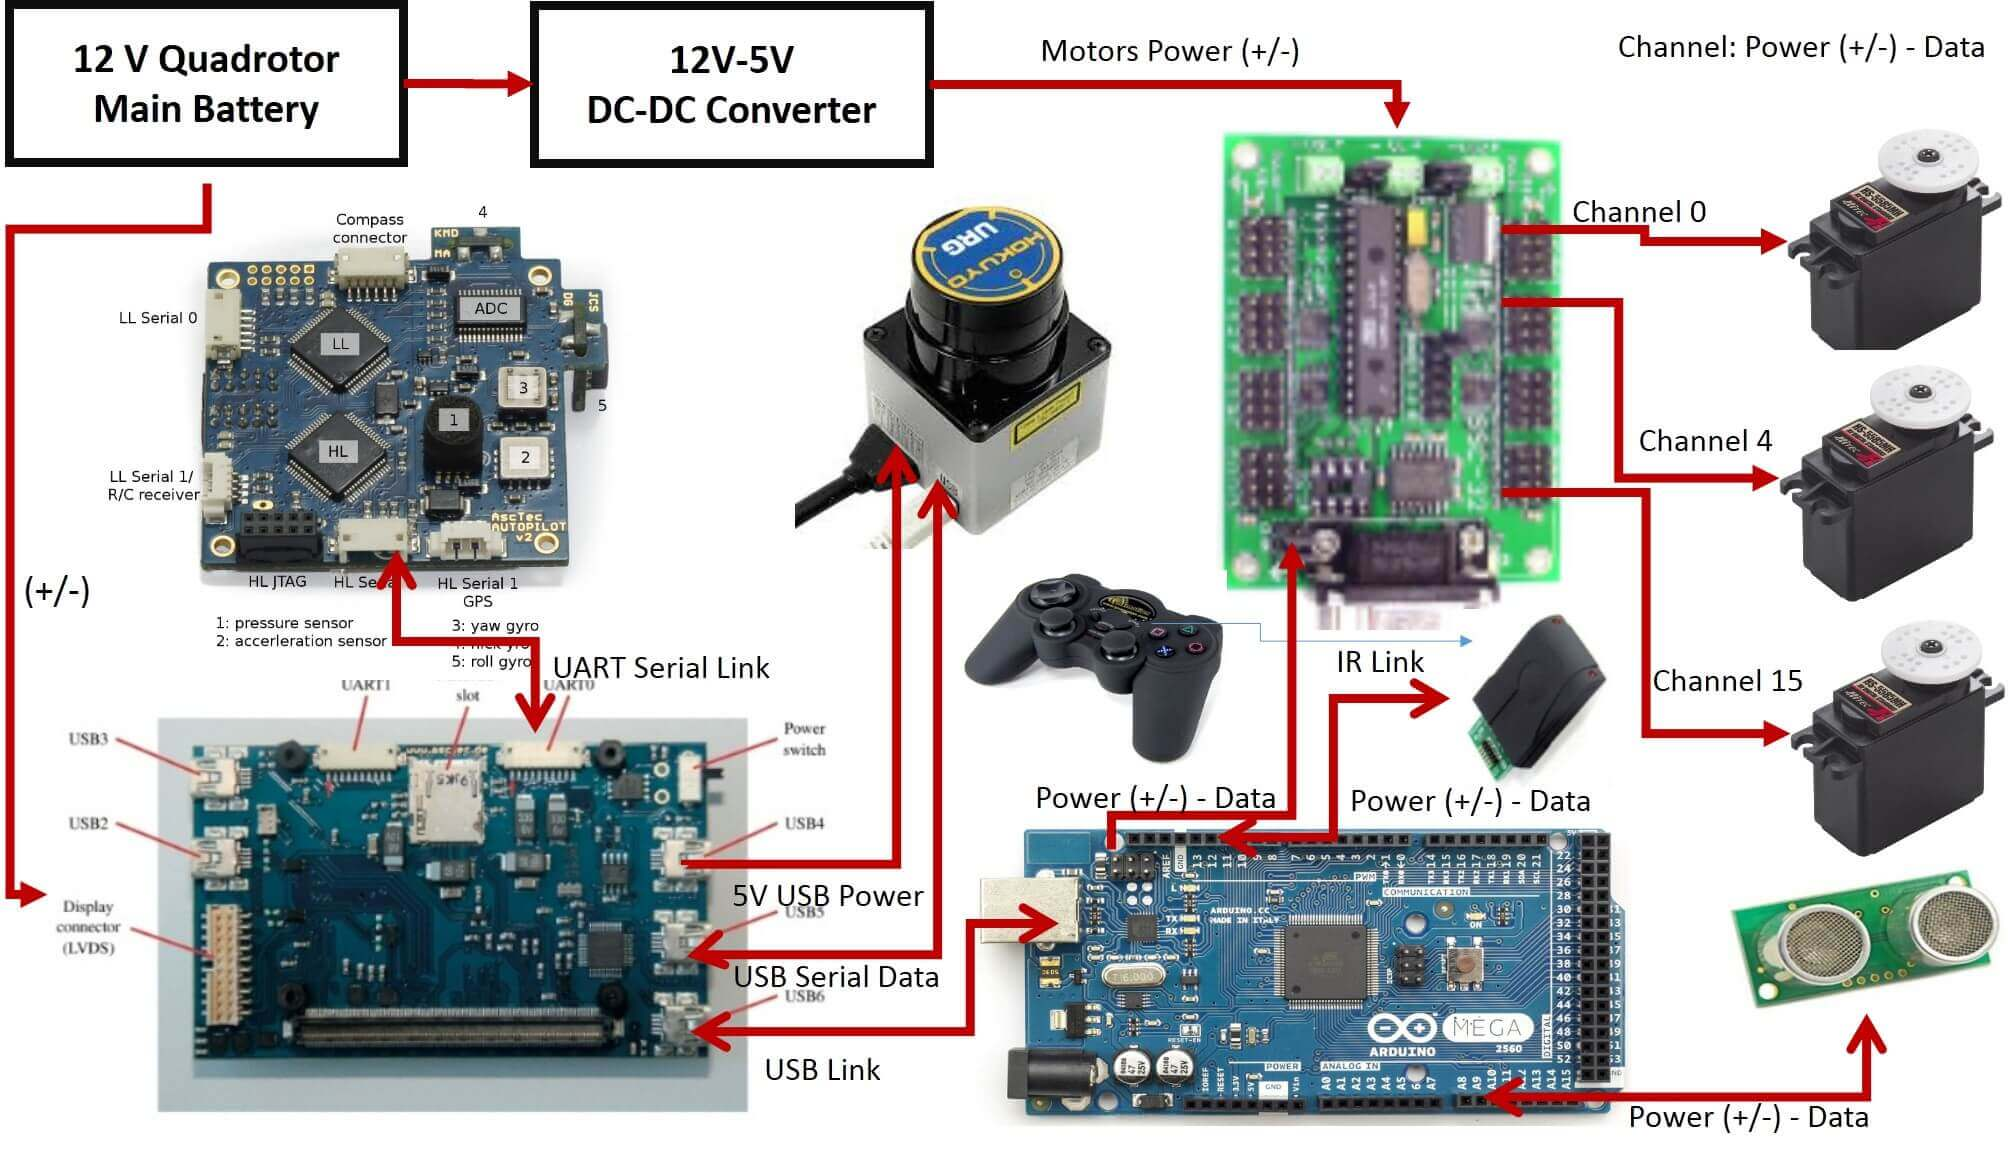}
	\caption{Power connections of the manipulator}
	\label{fig:power_conn}
\end{figure}
